# Supplementary material for: Versatile yet Efficient Network Traffic Analysis: Offloading Network Foundation Model to SmartNIC
Source: arXiv:2508.02001 source file (2026-11-12)
Supplement: Supplementary file 1 [file Address.tex]

\subsection{The Impact of Address-related Information}

\label{Address}

Since existing network foundation models follow the pre-training and fine-tuning paradigm, we examine the impact of address-related information across these two stages and make two experimental observations:


\begin{enumerate}
    \item In the pre-training stage, introducing address-related pre-training tasks leads to substantial inflation in downstream classification performance.
    
    \item In the fine-tuning stage, retaining address-related information yields spurious classification performance gains that do not survive simple protocol field randomization.
    
\end{enumerate}


\begin{figure}[h]
  \centering
  \includegraphics[width=0.8\linewidth]{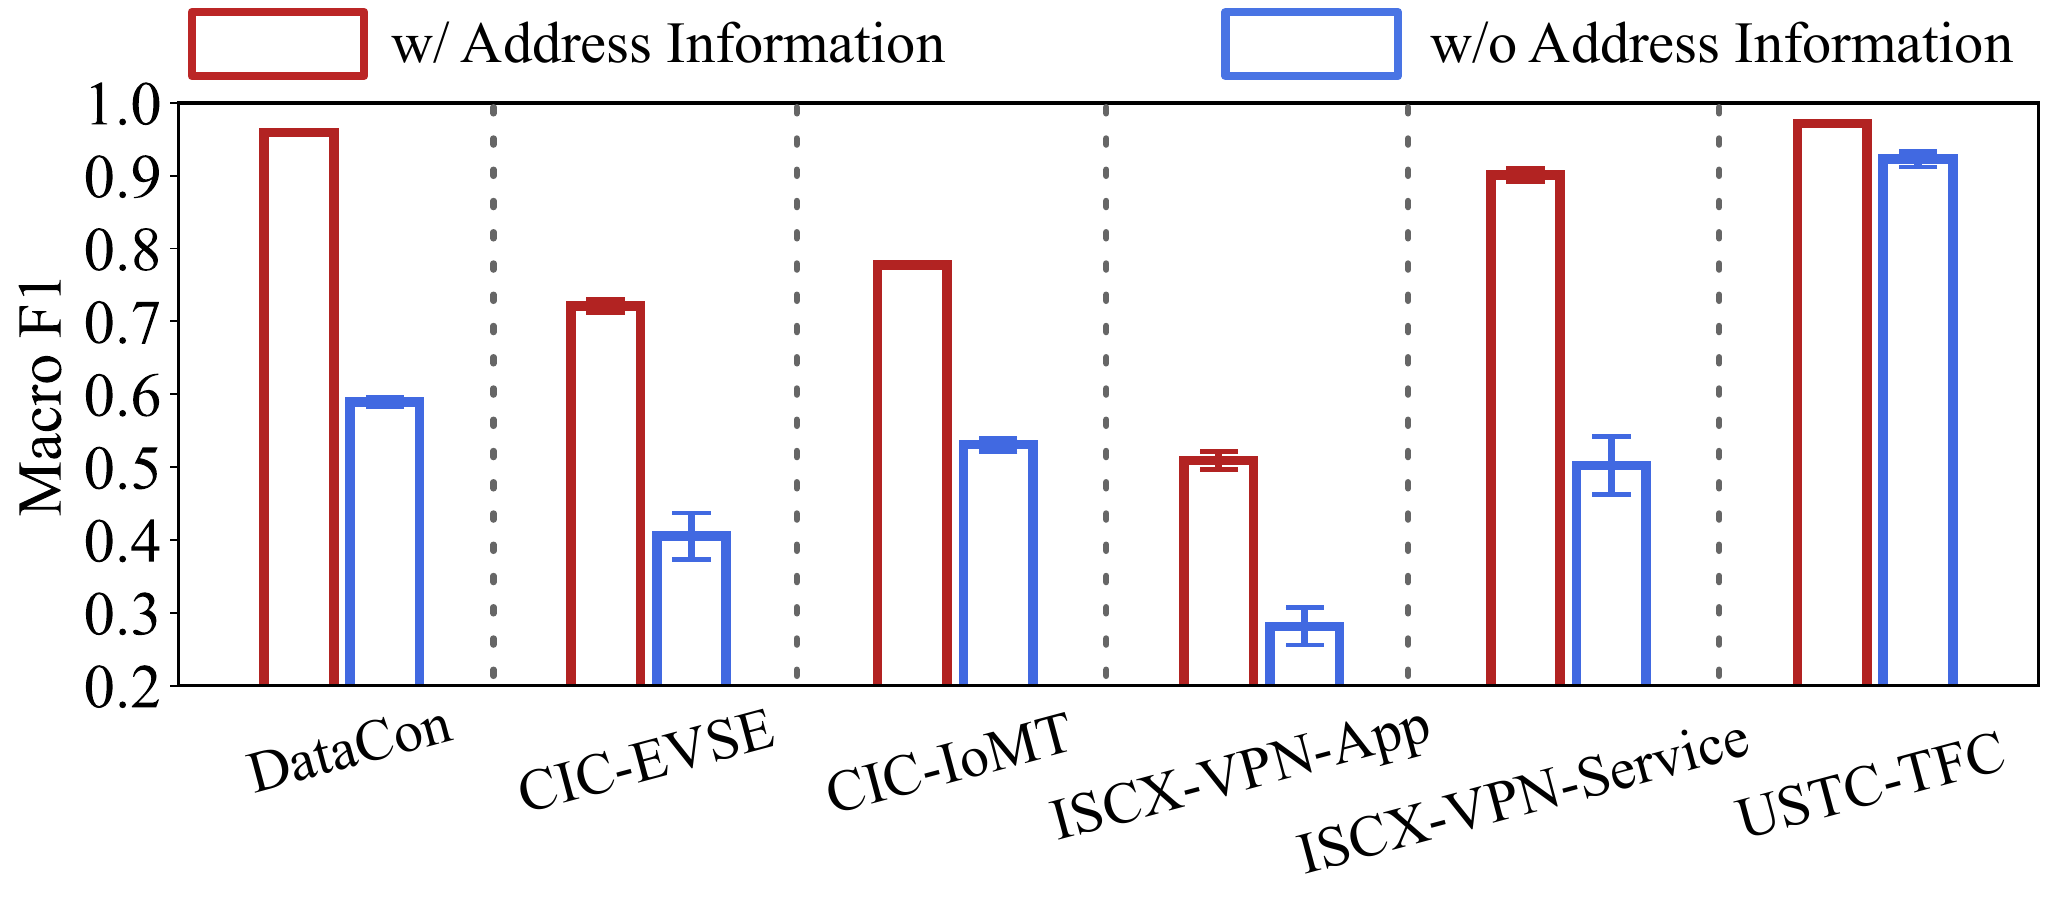}
  \caption{Impact of address-related pre-training tasks on Pcap-Encoder's performance across six traffic analysis tasks.}
  \vspace{-12pt}
  \label{fig:Address-Pretraining}
\end{figure}

In the pre-training stage, Pcap-Encoder \cite{Pcap-Encoder-SIGCOMM25} is the only network foundation model (to the best of our knowledge) that explicitly incorporates address-related information into its pre-training tasks, e.g., predicting the IP source/destination addresses of packets.
We pre-train two variants of Pcap-Encoder—with and without these tasks—and evaluate them on six traffic analysis tasks.
As shown in Fig. \ref{fig:Address-Pretraining}, removing them causes an average macro F1 drop of 34.69\%, e.g., from 0.9008 to 0.5020 on ISCX-VPN-Service.
This also explains Pcap-Encoder's lower performance in TABLE \ref{tab:Overall Classification Performance}, where all baselines are evaluated under our unbiased setting.

\begin{figure*}[t]
  \centering
  \includegraphics[width=\linewidth]{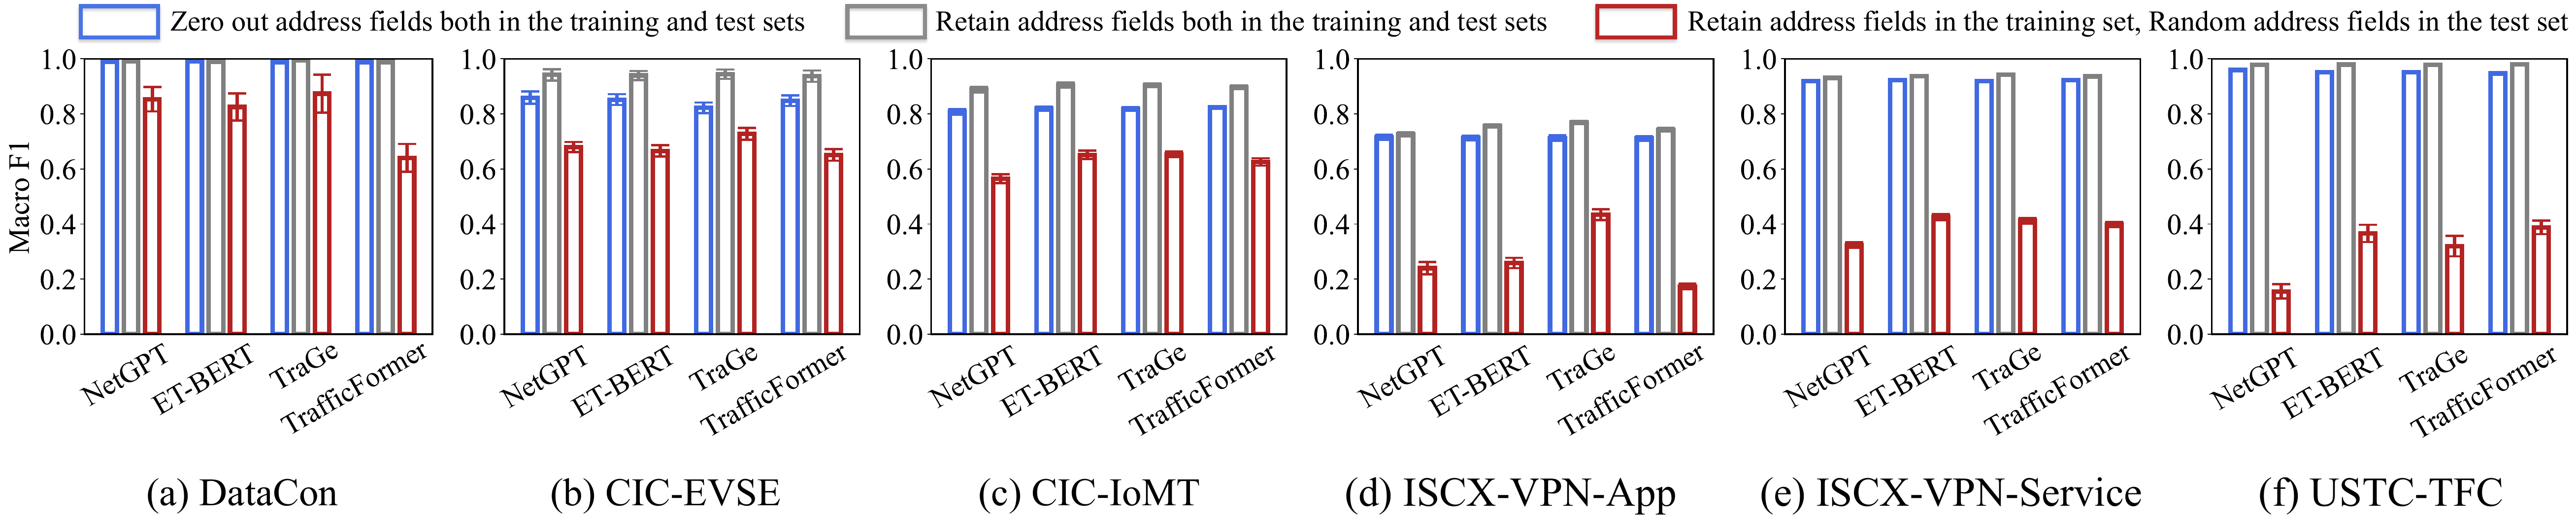}
  \caption{Impact of address-related information during the fine-tuning stage across six network traffic analysis tasks.}
  \vspace{-12pt}
  \label{fig:Address-Finetuning}
\end{figure*}


In the fine-tuning stage, we evaluate four network foundation models—NetGPT, ET-BERT, TraGe, and TrafficFormer—as TABLE \ref{tab:Overall Classification Performance} shows that they achieve markedly higher classification performance than other models.
We consider three settings: (i) zeroing out address-related fields in both training and test sets, (ii) retaining address-related fields in both, and (iii) retaining address-related fields in training but randomizing them in the test set.
As shown in Fig. \ref{fig:Address-Finetuning}, retaining address fields inflates macro F1 by 5.19\% on average over zeroing them out, but once test-time address fields are randomized, macro F1 drops by 44.67\% on average.
This sharp degradation indicates that the gains from retaining address fields stem from shortcut learning on address-related cues rather than from learning transferable traffic semantics.
Therefore, we zero out address-related protocol fields during traffic processing to ensure that the model learns transferable traffic semantics rather than address-related shortcuts, thereby providing unbiased estimates of generalization.
% Therefore, we zero out address-related fields to ensure unbiased generalization estimates.


% In the fine-tuning stage, we evaluate four network foundation models—NetGPT, ET-BERT, TraGe, and TrafficFormer—which achieve markedly higher performance than other models in TABLE~\ref{tab:Overall Classification Performance}.
% We consider three settings: (i) zeroing out address-related fields in both training and test sets, (ii) retaining them in both, and (iii) retaining them in training but randomizing them at test time.
% As shown in Fig.~\ref{fig:Address-Finetuning}, retaining address fields inflates macro F1 by 5.19\% on average over zeroing them out, but once test-time address fields are randomized, macro F1 drops by 44.67\% on average.
% This degradation indicates that the gains stem from shortcut learning on address-related cues rather than from transferable traffic semantics
