# Supplementary material for: Versatile yet Efficient Network Traffic Analysis: Offloading Network Foundation Model to SmartNIC
Source: arXiv:2508.02001 source file (2026-11-12)
Supplement: Supplementary file 2 [file Adversarial-Robustness.tex]

\subsection{\cg{Adversarial Robustness Evaluation}}

\label{Adversarial-Robustness}

\begin{figure}[t]
  \centering
  \includegraphics[width=1\linewidth]{Fig/Robustness/V2.pdf}
  \caption{\cg{Adversarial robustness evaluation of \textit{Nepco} and three Transformer-based network foundation models.}}
  \vspace{-8pt}
  \label{fig:Robustness}
\end{figure}


\cg{We conduct the adversarial robustness evaluation experiment on the CIC-EVSE dataset and compare \textit{Nepco} with three Transformer-based network foundation models, i.e., ET-BERT, TraGe, and TrafficFormer. For each model, we first train a model using the unperturbed training set. Based on the trained model, we apply gradient-based attribution \cite{gradient-arXiv17} to each sample in the training and test sets and rank its input bytes according to their attribution scores. We then construct two byte-level perturbation strategies. Random-X\% perturbation randomly selects X\% of the input bytes, while Top-X\% perturbation selects the top X\% most important bytes according to the byte importance ranking. Under both strategies, the selected bytes are replaced with random byte values. Based on the perturbed training and test sets, we consider four evaluation settings:}

\begin{itemize}[leftmargin=*]
\item \cg{\textbf{Raw-Random}: The model is trained on the unperturbed raw training set and evaluated on the Random-X\% test set.}
\item \cg{\textbf{Raw-Top}: The model is trained on the unperturbed raw training set and evaluated on the Top-X\% test set.}
\item \cg{\textbf{Random-Random}: The model is trained on the Random-X\% training set and evaluated on the Random-X\% test set.}
\item \cg{\textbf{Top-Top}: The model is trained on the Top-X\% training set and evaluated on the Top-X\% test set.}
\end{itemize}

\cg{The dashed lines in Fig. \ref{fig:Robustness} show the macro F1 of different models when the test samples are perturbed by Random-X\% and Top-X\% perturbations, corresponding to the Raw-Random and Raw-Top settings, respectively, while the gray lines show the macro F1 when the test samples are not perturbed.
Under Random-X\% perturbation, the macro F1 degradation is limited. Over the perturbation range from 0\% to 5\%, each 1-percentage-point increase in X corresponds to average macro F1 reductions of 0.0098, 0.0143, 0.0096, and 0.0037 for \textit{Nepco}, TrafficFormer, TraGe, and ET-BERT, respectively.
Under Top-X\% perturbation, the macro F1 decreases substantially as X increases, with corresponding average reductions of 0.0878, 0.0951, 0.0951, and 0.0953.
These results show that the four models are sensitive to perturbations of high-importance bytes, while \textit{Nepco} does not exhibit greater sensitivity than the three Transformer-based models.}

\cg{The solid lines in Fig. \ref{fig:Robustness} show the macro F1 of different models when both the training and test samples are perturbed by Random-X\% and Top-X\% perturbations, corresponding to the Random-Random and Top-Top settings, respectively.
Under both strategies, introducing the corresponding perturbations during training substantially mitigates the performance degradation caused by test-time perturbations, with the four models maintaining macro F1 above 0.84 across the evaluated perturbation ratios.
Specifically, under Top-5\% perturbation, the macro F1 of \textit{Nepco}, TrafficFormer, TraGe, and ET-BERT are 0.8447, 0.9082, 0.8987, and 0.8918, respectively.}
