# Supplementary material for: Versatile yet Efficient Network Traffic Analysis: Offloading Network Foundation Model to SmartNIC
Source: arXiv:2508.02001 source file (2026-11-12)
Supplement: Supplementary file 3 [file Local-Pattern.tex]

% \clearpage

\subsection{Cross-Dataset Localized Byte-sequence Pattern}

\label{Local-Pattern}

We further examine localized byte-sequence patterns across datasets through quantitative analysis, providing additional support for the four observations in Section \ref{sec:Localized Pattern-Aware Traffic Modeling}.
As conducting this analysis on every public dataset is infeasible, we select two representative datasets, i.e., USTC-TFC, which is part of our fine-tuning evaluation, and CIC-IoT, which is held out from both pre-training and fine-tuning, covering both in-evaluation and out-of-evaluation settings.
We present four observation supports (\textbf{OS1–OS4}), each providing quantitative analysis for the corresponding observation (\textbf{O1–O4}).




\begin{figure}[t]
  \centering
  \includegraphics[width=1\linewidth]{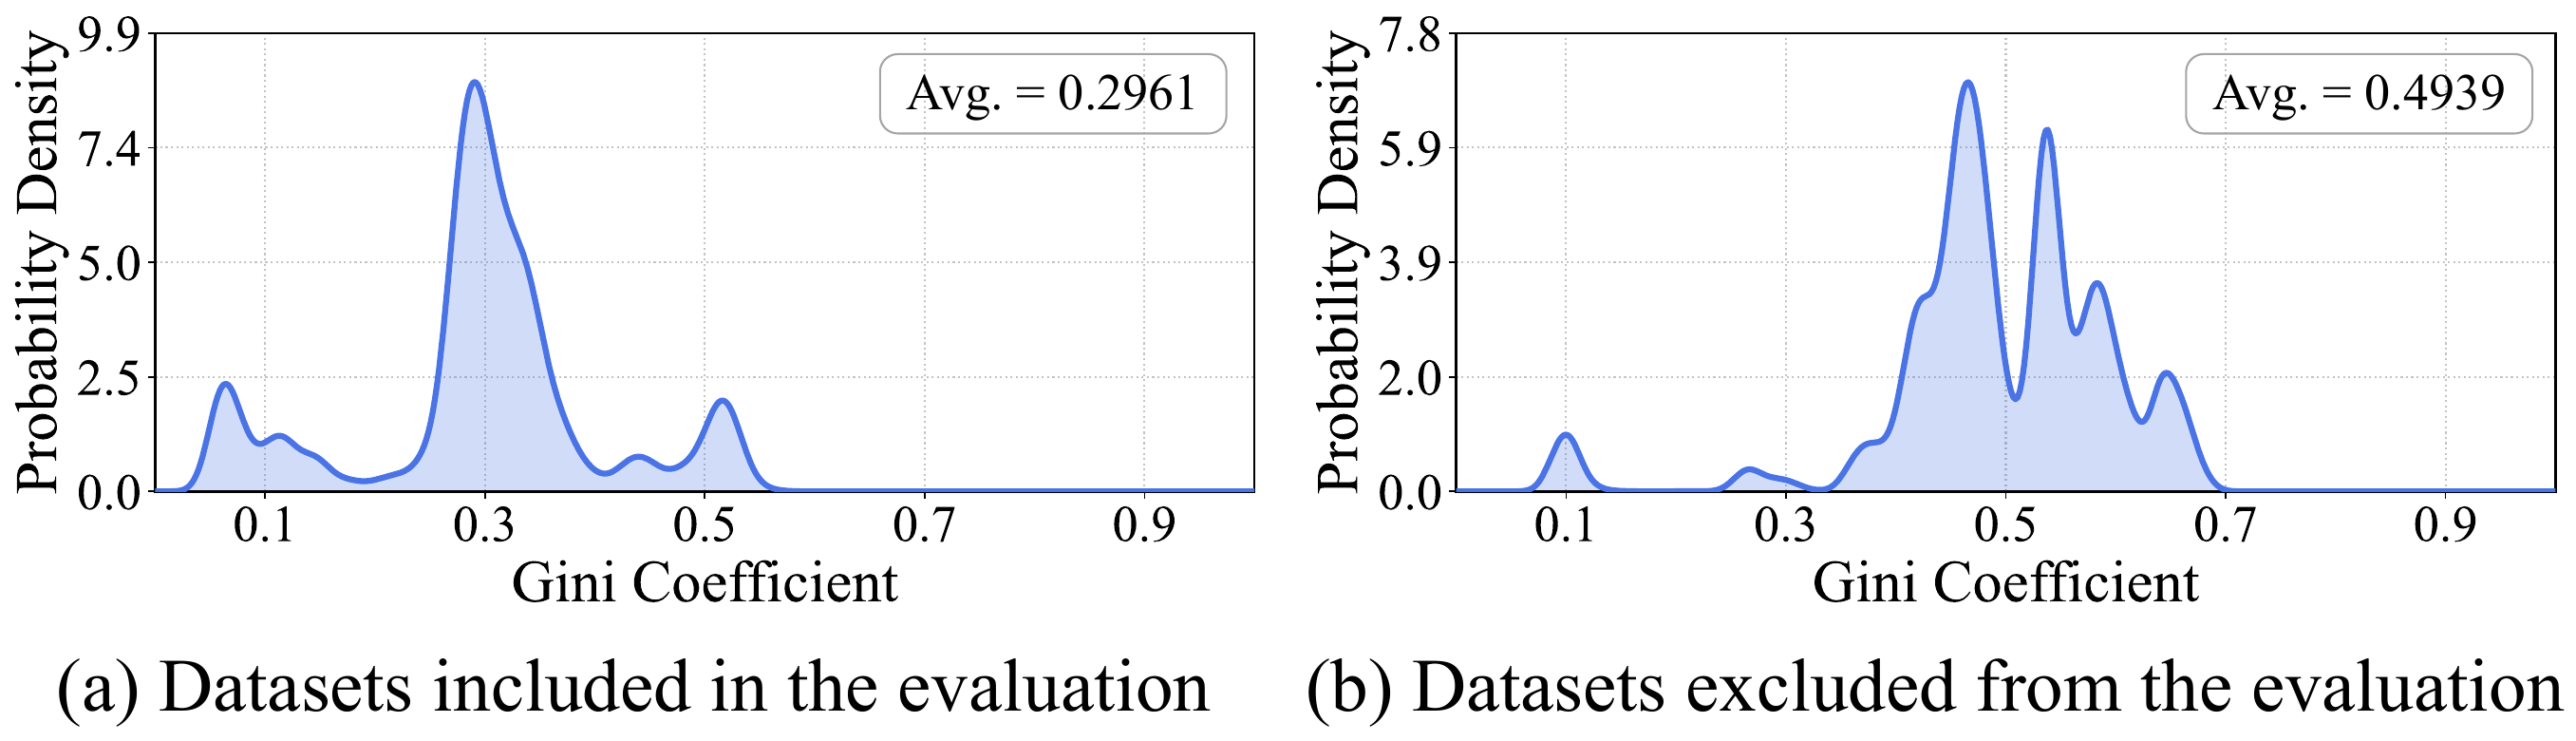}
  \caption{Distribution of Gini coefficients computed on byte importance score sequences.}
  \vspace{-10pt}
  \label{fig:Gini}
\end{figure}


\begin{figure}[t]
  \centering
  \includegraphics[width=1\linewidth]{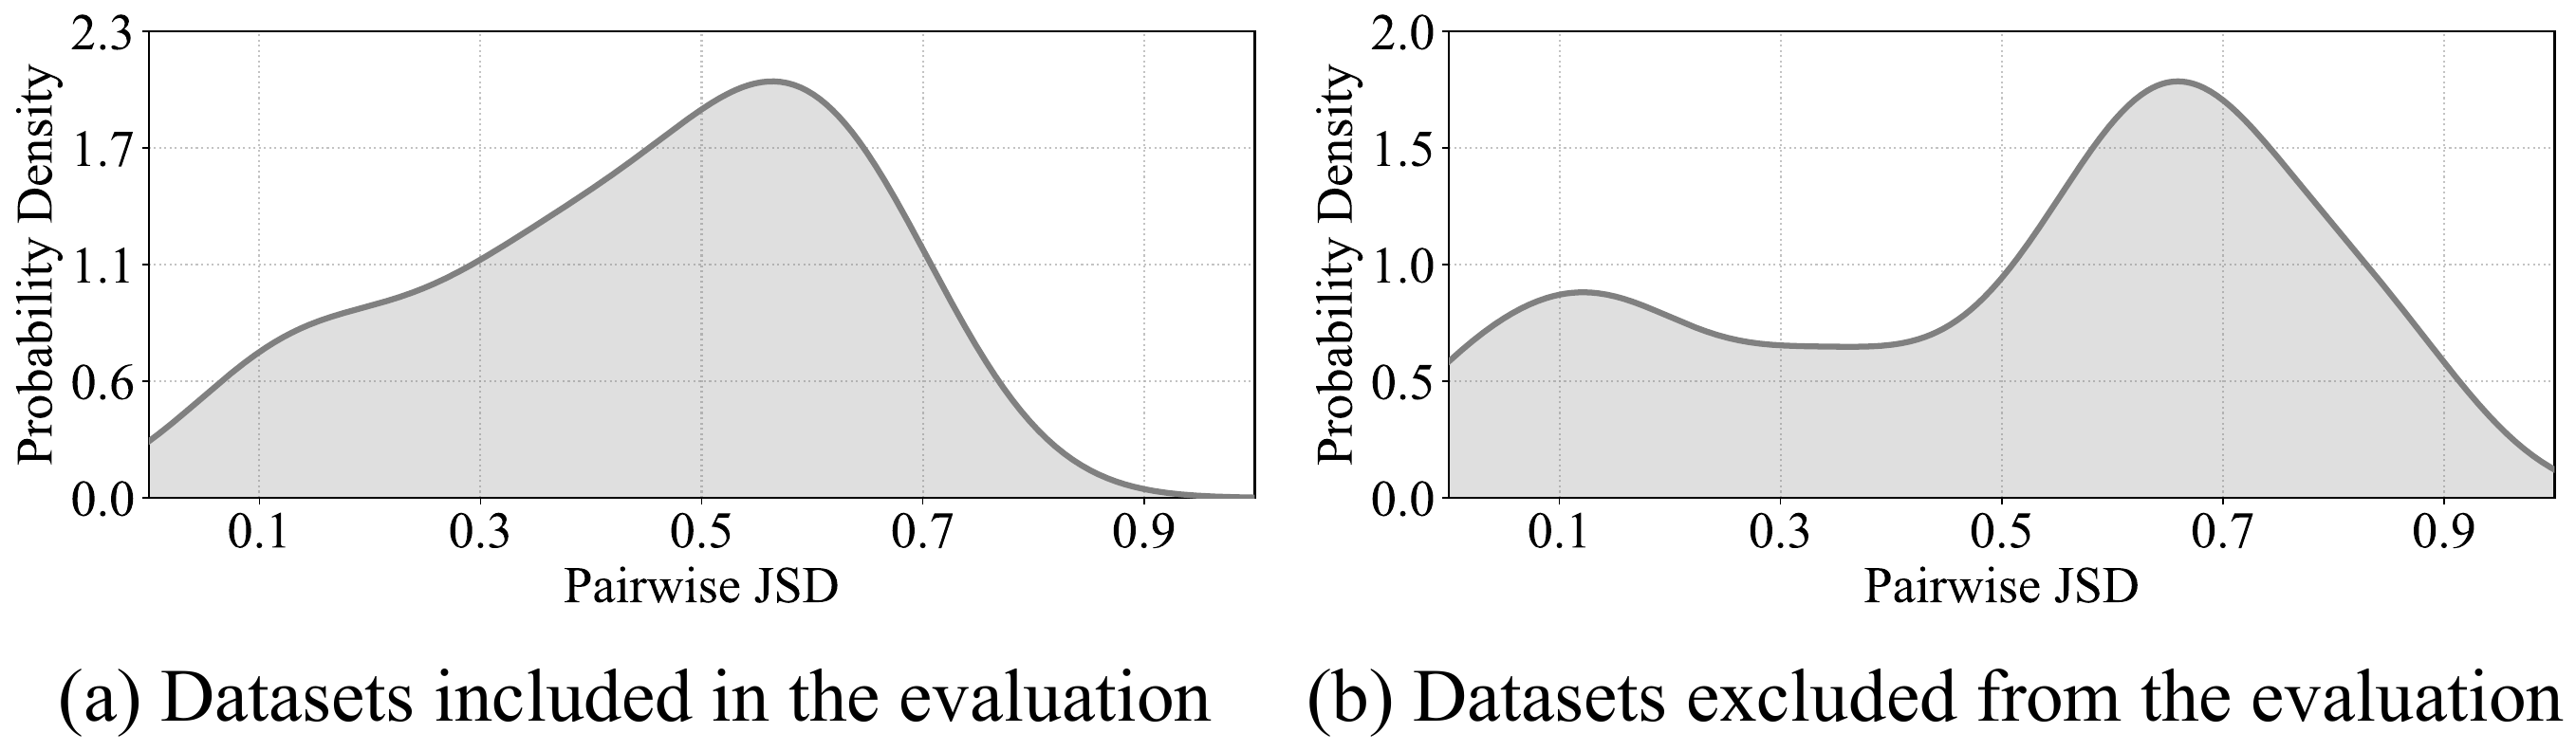}
  \caption{Distribution of pairwise Jensen-Shannon Divergence between per-class field distributions.}
  \vspace{-10pt}
  \label{fig:Pair-JSD}
\end{figure}

% \vspace{0.05in}
\noindent\textbf{\cg{OS1: Discriminative traffic patterns are often localized.}}
% We compute the Gini coefficient \cite{Gini} of the byte importance score sequences, which quantifies how unevenly the importance is distributed: a value close to 0 means importance is spread across all bytes, while a value close to 1 means a few bytes hold most of the importance.
% In Fig.~\ref{fig:Gini}, the per-packet Gini is centered above zero on both datasets (Fig.~\ref{fig:Gini}(a), averaging 0.2961; Fig.~\ref{fig:Gini}(b), averaging 0.4939), indicating that byte importance is concentrated on a small subset of positions.
We compute the Gini coefficient \cite{Gini} of the byte importance score sequences to quantify how unevenly importance is distributed across byte positions.
A value close to 0 indicates uniform distribution, while a value close to 1 indicates concentration on a few bytes.
As shown in Fig.~\ref{fig:Gini}, the Gini distributions are right-skewed and consistently centered above zero on both datasets, averaging 0.2961 on USTC-TFC (Fig.~\ref{fig:Gini}(a)) and 0.4939 on CIC-IoT (Fig.~\ref{fig:Gini}(b)).
% The right-skewed shape indicates that the majority of traffic samples exhibit meaningful locality rather than a small fraction of outliers driving the average upward, confirming that byte importance concentration is a general property of network traffic rather than an artifact of any particular dataset.
\cg{This distribution provides evidence that byte importance is non-uniform and often concentrated on subsets of byte positions rather than being uniformly distributed across the sequence. This provides cross-dataset support for the locality observation, suggesting that it is not limited to a single evaluation dataset.}


% \vspace{0.05in}
\noindent\textbf{\cg{OS2: Different categories favor different local regions.}}
% For each packet, we identify its Top-5 most important protocol fields and aggregate per-class field distributions.
% We then compute the pairwise Jensen-Shannon Divergence (JSD) \cite{JSD} between every pair of classes, where a higher JSD indicates more divergent field preferences.
% In Fig.~\ref{fig:Pair-JSD}, the pairwise JSD is above zero on both datasets, indicating that distinct classes rely on substantially different sets of protocol fields.
For each traffic sample, we identify its Top-5 most important protocol fields and aggregate the field-level importance distribution per class.
We then compute the pairwise Jensen-Shannon Divergence (JSD) \cite{JSD} between per-class distributions for every pair of classes, where a higher JSD indicates more divergent field preferences.
As shown in Fig.~\ref{fig:Pair-JSD}, the pairwise JSD distribution is consistently above zero across all class pairs on both datasets, with the bulk of mass concentrated at moderate-to-high divergence values. 
% This confirms that distinct traffic classes concentrate their importance on substantially different protocol field regions, validating that localized modeling retains sufficient discriminative capacity for multi-class analysis.
\cg{This provides evidence that different traffic classes may rely on discriminative information located in different field regions.}

% \vspace{0.05in}
\noindent\textbf{\cg{OS3: Discriminative bytes often occupy only part of a field.}}
% For each packet, we identify the protocol fields hit by its Top-5 most important bytes, and compute the Gini coefficient on the byte importance score sequence within each hit field.
% As shown in Fig.~\ref{fig:Gini-Field}, the field-level Gini is above zero on both datasets (Fig.~\ref{fig:Gini-Field}(a), averaging 0.2907; Fig.~\ref{fig:Gini-Field}(b), averaging 0.4389), indicating that even within high-importance fields, only a subset of bytes is highly weighted.
For each traffic sample, we identify the protocol fields hit by its Top-5 most important bytes and compute the Gini coefficient over the byte importance scores within each such field.
As shown in Fig.~\ref{fig:Gini-Field}, the field-level Gini is consistently above zero on both datasets, averaging 0.2907 on USTC-TFC (Fig.~\ref{fig:Gini-Field}(a)) and 0.4389 on CIC-IoT (Fig.~\ref{fig:Gini-Field}(b)), indicating that even within high-importance protocol fields, only a subset of bytes is highly weighted.
% This intra-field selectivity motivates the window-wise byte scoring in \textit{Nepco}, which assigns learnable per-position weights within each convolution window rather than treating all bytes uniformly.



% \vspace{0.05in}
\noindent\textbf{OS4: Address fields attract disproportionate importance.}
% For each packet, we measure how often each of the eight address-related fields is hit by its Top-5 most important bytes, and report the \textit{At-Least-One Hit@5} metric—the fraction of packets in which at least one address-related field is hit.
% As shown in Fig.~\ref{fig:Address_Hit}, the metric reaches 0.8816 on Fig.~\ref{fig:Address_Hit}(a) and 0.9675 on Fig.~\ref{fig:Address_Hit}(b), indicating that without address zeroing, the model's importance is dominated by address-related fields.
For each traffic sample, we measure how often each of the eight address-related protocol fields is hit by its Top-5 most important bytes, and report the At-Least-One Hit@5 metric, defined as the fraction of traffic samples in which at least one address-related field is hit.
As shown in Fig.~\ref{fig:Address_Hit}, the metric reaches 0.8816 on USTC-TFC (Fig.~\ref{fig:Address_Hit}(a)) and 0.9675 on CIC-IoT (Fig.~\ref{fig:Address_Hit}(b)), indicating that without address zeroing, address-related fields dominate byte importance in the vast majority of traffic samples. Since these fields carry no transferable traffic semantics, this confirms that address zeroing is necessary not only for evaluation validity but also to redirect the model toward learning class-discriminative traffic patterns.


\begin{figure}[t]
  \centering
  \includegraphics[width=1\linewidth]{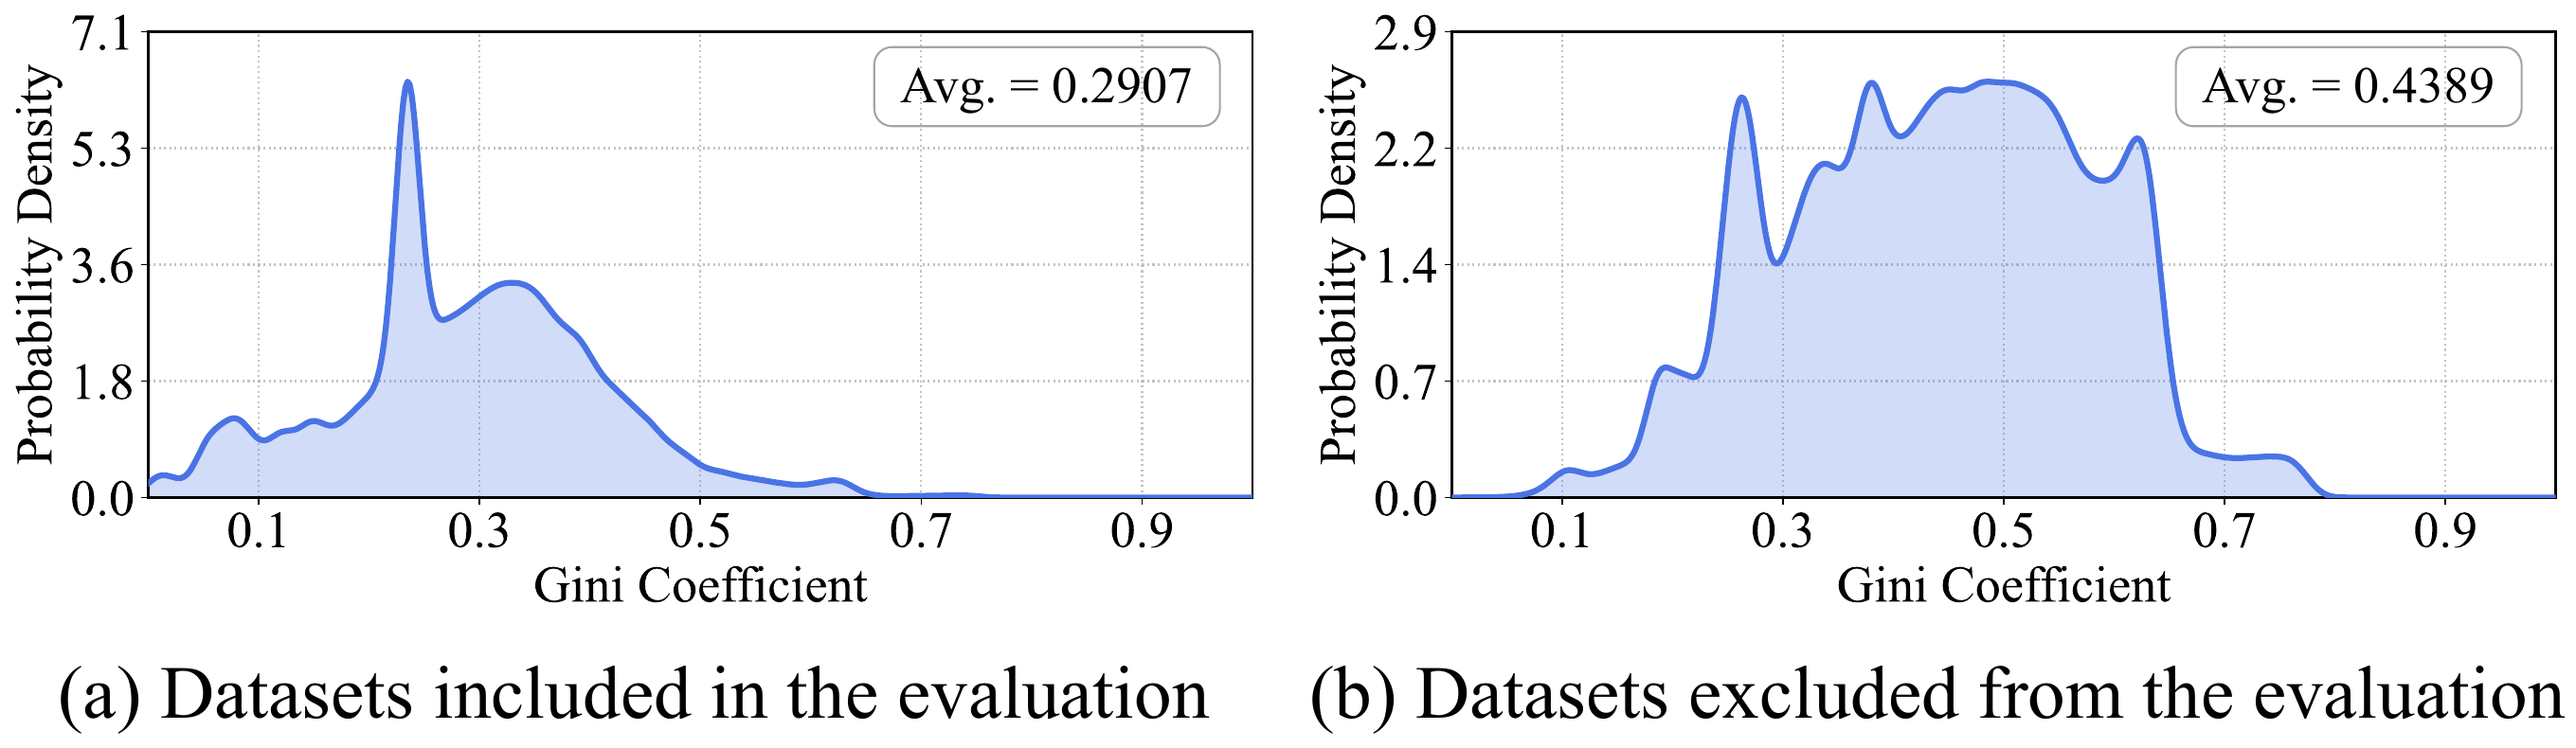}
  \caption{Distribution of per-sequence Gini coefficients of byte importance scores within each Top-5 protocol field.}
  \vspace{-10pt}
  \label{fig:Gini-Field}
\end{figure}



\begin{figure}[t]
  \centering
  \includegraphics[width=1\linewidth]{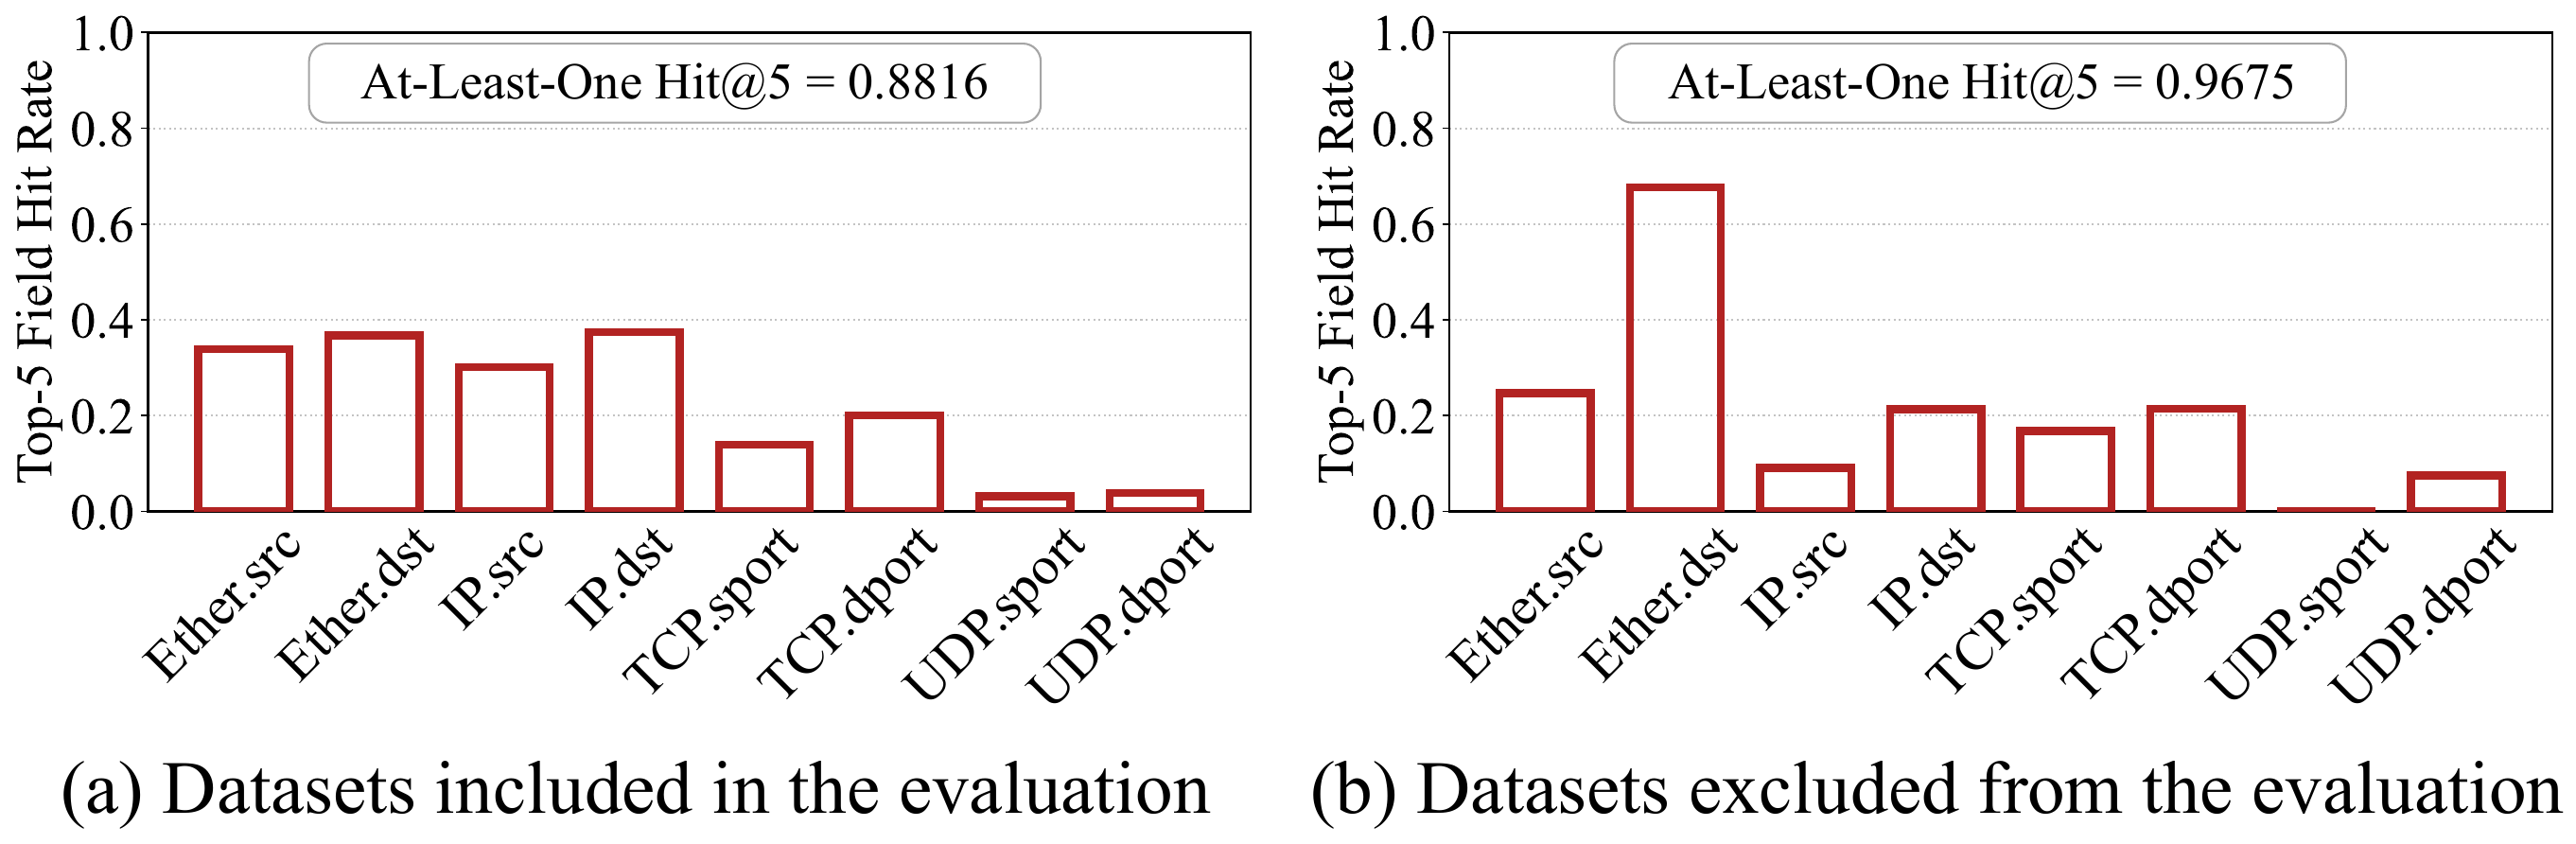}
  \caption{Hit frequency of eight address-related protocol fields in the Top-5 most important bytes.}
  \vspace{-10pt}
  \label{fig:Address_Hit}
\end{figure}
