# Supplementary material for: Versatile yet Efficient Network Traffic Analysis: Offloading Network Foundation Model to SmartNIC
Source: arXiv:2508.02001 source file (2026-11-12)
Supplement: Supplementary file 4 [file New_Dataset.tex]

\subsection{\cg{Evaluation on Three More Network Traffic Datasets}}

\label{New_Dataset}

\begin{table*}[t!]
\renewcommand{\arraystretch}{1.1}
\centering
\small
\caption{\cg{The overall classification performances of \textit{Nepco} and baselines on three more network traffic datasets.}}
\label{tab:Additional Classification Performance}
\resizebox{1\textwidth}{!}{%
\begin{tabular}{c|c|ccc|ccc|ccc}

\toprule
\multicolumn{2}{c|}{\multirow{2}{*}{\textbf{Method} \textsuperscript{1}}} &
\multicolumn{3}{c|}{\textbf{CSTNET-20 (2023)}} &
\multicolumn{3}{c|}{\textbf{CSTNET-120 (2023)}} &
\multicolumn{3}{c}{\textbf{DoHBrw (2020)}} \\

\multicolumn{2}{c|}{} &
Precision &
Recall &
Macro F1 &
Precision &
Recall &
Macro F1 &
Precision &
Recall &
Macro F1 \\ \midrule

\multirow{9}{*}{\rotatebox[origin=c]{90}{\makecell{ML/DL Model \\ \textbf{\textcolor{CheckBlue}{\ding{51}}}: Hardware-Offloadable}}} &
FlowPrint &
0.0992 {\scriptsize\(\pm \ 0.0110\)} &
0.1314 {\scriptsize\(\pm \ 0.0124\)} &
0.0971 {\scriptsize\(\pm \ 0.0108\)} &
0.0953 {\scriptsize\(\pm \ 0.0043\)} &
0.1023 {\scriptsize\(\pm \ 0.0025\)} &
0.0850 {\scriptsize\(\pm \ 0.0027\)} &
0.2843 {\scriptsize\(\pm \ 0.0244\)} &
0.3120 {\scriptsize\(\pm \ 0.0195\)} &
0.2853 {\scriptsize\(\pm \ 0.0213\)} \\

 &
AppScanner &
0.6962 {\scriptsize\(\pm \ 0.0024\)} &
0.6809 {\scriptsize\(\pm \ 0.0024\)} &
0.6825 {\scriptsize\(\pm \ 0.0024\)} &
0.5571 {\scriptsize\(\pm \ 0.0018\)} &
0.5002 {\scriptsize\(\pm \ 0.0012\)} &
0.5148 {\scriptsize\(\pm \ 0.0012\)} &
0.4749 {\scriptsize\(\pm \ 0.0015\)} &
0.4586 {\scriptsize\(\pm \ 0.0016\)} &
0.4560 {\scriptsize\(\pm \ 0.0014\)} \\

 &
XGBoost &
0.6921 {\scriptsize\(\pm \ 0.0248\)} &
0.6637 {\scriptsize\(\pm \ 0.0329\)} &
0.6795 {\scriptsize\(\pm \ 0.0214\)} &
0.2985 {\scriptsize\(\pm \ 0.0185\)} &
0.2851 {\scriptsize\(\pm \ 0.0164\)} &
0.2818 {\scriptsize\(\pm \ 0.0183\)} &
0.4652 {\scriptsize\(\pm \ 0.0114\)} &
0.4367 {\scriptsize\(\pm \ 0.0157\)} &
0.4412 {\scriptsize\(\pm \ 0.0148\)} \\

 &
DTree &
0.5628 {\scriptsize\(\pm \ 0.0341\)} &
0.5324 {\scriptsize\(\pm \ 0.0413\)} &
0.5515 {\scriptsize\(\pm \ 0.0409\)} &
0.2124 {\scriptsize\(\pm \ 0.0103\)} &
0.2021 {\scriptsize\(\pm \ 0.0198\)} &
0.2097 {\scriptsize\(\pm \ 0.0125\)} &
0.4113 {\scriptsize\(\pm \ 0.0123\)} &
0.4067 {\scriptsize\(\pm \ 0.0196\)} &
0.4119 {\scriptsize\(\pm \ 0.0187\)} \\

 &
Flowrest \textbf{\textcolor{CheckBlue}{\ding{51}}} &
\textbf{\textcolor{CheckBlue}{\uline{0.7161 {\scriptsize\(\pm \ 0.0142\)}}}} &
\textbf{\textcolor{CheckBlue}{\uline{0.6857 {\scriptsize\(\pm \ 0.0081\)}}}} &
\textbf{\textcolor{CheckBlue}{\uline{0.6803 {\scriptsize\(\pm \ 0.0098\)}}}} &
0.3297 {\scriptsize\(\pm \ 0.0099\)} &
\textbf{\textcolor{CheckBlue}{\uline{0.2980 {\scriptsize\(\pm \ 0.0043\)}}}} &
\textbf{\textcolor{CheckBlue}{\uline{0.2659 {\scriptsize\(\pm \ 0.0054\)}}}} &
\textbf{\textcolor{CheckBlue}{\uline{0.5354 {\scriptsize\(\pm \ 0.0032\)}}}} &
\textbf{\textcolor{CheckBlue}{\uline{0.5367 {\scriptsize\(\pm \ 0.0039\)}}}} &
\textbf{\textcolor{CheckBlue}{\uline{0.5322 {\scriptsize\(\pm \ 0.0040\)}}}} \\

 &
Leo \textbf{\textcolor{CheckBlue}{\ding{51}}} &
0.2986 {\scriptsize\(\pm \ 0.0106\)} &
0.3901 {\scriptsize\(\pm \ 0.0055\)} &
0.3142 {\scriptsize\(\pm \ 0.0074\)} &
0.0211 {\scriptsize\(\pm \ 0.0003\)} &
0.0993 {\scriptsize\(\pm \ 0.0010\)} &
0.0330 {\scriptsize\(\pm \ 0.0004\)} &
0.4412 {\scriptsize\(\pm \ 0.0215\)} &
0.4470 {\scriptsize\(\pm \ 0.0053\)} &
0.4128 {\scriptsize\(\pm \ 0.0085\)} \\

 &
Mousika \textbf{\textcolor{CheckBlue}{\ding{51}}} &
0.6151 {\scriptsize\(\pm \ 0.0202\)} &
0.4896 {\scriptsize\(\pm \ 0.0086\)} &
0.4725 {\scriptsize\(\pm \ 0.0107\)} &
\textbf{\textcolor{CheckBlue}{\uline{0.3752 {\scriptsize\(\pm \ 0.0062\)}}}} &
0.2580 {\scriptsize\(\pm \ 0.0020\)} &
0.2412 {\scriptsize\(\pm \ 0.0019\)} &
0.3922 {\scriptsize\(\pm \ 0.0372\)} &
0.4403 {\scriptsize\(\pm \ 0.0025\)} &
0.3587 {\scriptsize\(\pm \ 0.0018\)} \\

 &
EBSNN &
0.8234 {\scriptsize\(\pm \ 0.0404\)} &
0.7915 {\scriptsize\(\pm \ 0.0438\)} &
0.7819 {\scriptsize\(\pm \ 0.0475\)} &
0.6052 {\scriptsize\(\pm \ 0.0274\)} &
0.5600 {\scriptsize\(\pm \ 0.0256\)} &
0.5426 {\scriptsize\(\pm \ 0.0281\)} &
0.5354 {\scriptsize\(\pm \ 0.0302\)} &
0.5139 {\scriptsize\(\pm \ 0.0178\)} &
0.4897 {\scriptsize\(\pm \ 0.0277\)} \\

 &
BoS \textbf{\textcolor{CheckBlue}{\ding{51}}} &
0.3370 {\scriptsize\(\pm \ 0.0136\)} &
0.3795 {\scriptsize\(\pm \ 0.0167\)} &
0.3815 {\scriptsize\(\pm \ 0.0125\)} &
0.0183 {\scriptsize\(\pm \ 0.0012\)} &
0.0175 {\scriptsize\(\pm \ 0.0018\)} &
0.0446 {\scriptsize\(\pm \ 0.0023\)} &
0.4103 {\scriptsize\(\pm \ 0.0070\)} &
0.4113 {\scriptsize\(\pm \ 0.0158\)} &
0.4559 {\scriptsize\(\pm \ 0.0038\)} \\

\midrule

\multirow{9}{*}{\rotatebox[origin=c]{90}{\makecell{Network Foundation Model \\ \textbf{\textcolor{CheckBlue}{\ding{51}}}: Hardware-Offloadable}}} &
NetMamba &
0.8672 {\scriptsize\(\pm \ 0.0104\)} &
0.8393 {\scriptsize\(\pm \ 0.0093\)} &
0.8435 {\scriptsize\(\pm \ 0.0100\)} &
0.4246 {\scriptsize\(\pm \ 0.0735\)} &
0.4256 {\scriptsize\(\pm \ 0.0742\)} &
0.3947 {\scriptsize\(\pm \ 0.0689\)} &
0.5474 {\scriptsize\(\pm \ 0.0077\)} &
0.5380 {\scriptsize\(\pm \ 0.0056\)} &
0.5316 {\scriptsize\(\pm \ 0.0051\)} \\

 &
YaTC &
0.8293 {\scriptsize\(\pm \ 0.0054\)} &
0.8309 {\scriptsize\(\pm \ 0.0056\)} &
0.8122 {\scriptsize\(\pm \ 0.0056\)} &
0.6013 {\scriptsize\(\pm \ 0.0057\)} &
0.5834 {\scriptsize\(\pm \ 0.0039\)} &
0.5621 {\scriptsize\(\pm \ 0.0044\)} &
0.5516 {\scriptsize\(\pm \ 0.0051\)} &
0.5394 {\scriptsize\(\pm \ 0.0050\)} &
0.5398 {\scriptsize\(\pm \ 0.0052\)} \\

 &
Pcap-Encoder &
0.7417 {\scriptsize\(\pm \ 0.0152\)} &
0.7486 {\scriptsize\(\pm \ 0.0092\)} &
0.7370 {\scriptsize\(\pm \ 0.0110\)} &
0.3076 {\scriptsize\(\pm \ 0.0044\)} &
0.3909 {\scriptsize\(\pm \ 0.0034\)} &
0.3334 {\scriptsize\(\pm \ 0.0041\)} &
0.4770 {\scriptsize\(\pm \ 0.0044\)} &
0.4752 {\scriptsize\(\pm \ 0.0040\)} &
0.4737 {\scriptsize\(\pm \ 0.0042\)} \\

 &
PERT &
0.9001 {\scriptsize\(\pm \ 0.0090\)} &
0.8770 {\scriptsize\(\pm \ 0.0039\)} &
0.8703 {\scriptsize\(\pm \ 0.0050\)} &
0.6638 {\scriptsize\(\pm \ 0.0047\)} &
0.6151 {\scriptsize\(\pm \ 0.0025\)} &
0.6123 {\scriptsize\(\pm \ 0.0027\)} &
0.6258 {\scriptsize\(\pm \ 0.0057\)} &
0.6215 {\scriptsize\(\pm \ 0.0056\)} &
0.6213 {\scriptsize\(\pm \ 0.0056\)} \\

 &
NetGPT &
0.9025 {\scriptsize\(\pm \ 0.0064\)} &
0.8775 {\scriptsize\(\pm \ 0.0038\)} &
0.8702 {\scriptsize\(\pm \ 0.0041\)} &
0.6367 {\scriptsize\(\pm \ 0.0047\)} &
0.5934 {\scriptsize\(\pm \ 0.0034\)} &
0.5876 {\scriptsize\(\pm \ 0.0036\)} &
0.6167 {\scriptsize\(\pm \ 0.0046\)} &
0.6064 {\scriptsize\(\pm \ 0.0040\)} &
0.6060 {\scriptsize\(\pm \ 0.0037\)} \\

 &
ET-BERT &
0.9026 {\scriptsize\(\pm \ 0.0085\)} &
0.8788 {\scriptsize\(\pm \ 0.0041\)} &
0.8707 {\scriptsize\(\pm \ 0.0046\)} &
0.6562 {\scriptsize\(\pm \ 0.0044\)} &
0.6128 {\scriptsize\(\pm \ 0.0033\)} &
0.6082 {\scriptsize\(\pm \ 0.0036\)} &
0.6317 {\scriptsize\(\pm \ 0.0040\)} &
0.6274 {\scriptsize\(\pm \ 0.0038\)} &
0.6277 {\scriptsize\(\pm \ 0.0039\)} \\

 &
TraGe &
0.8823 {\scriptsize\(\pm \ 0.0064\)} &
0.8759 {\scriptsize\(\pm \ 0.0027\)} &
0.8674 {\scriptsize\(\pm \ 0.0035\)} &
0.6623 {\scriptsize\(\pm \ 0.0050\)} &
0.6189 {\scriptsize\(\pm \ 0.0025\)} &
0.6161 {\scriptsize\(\pm \ 0.0028\)} &
0.6319 {\scriptsize\(\pm \ 0.0066\)} &
0.6208 {\scriptsize\(\pm \ 0.0068\)} &
0.6220 {\scriptsize\(\pm \ 0.0074\)} \\

 &
TrafficFormer &
\textbf{\textcolor{CrossRed}{0.9033 {\scriptsize\(\pm \ 0.0070\)}}} &
\textbf{\textcolor{CrossRed}{0.8789 {\scriptsize\(\pm \ 0.0045\)}}} &
\textbf{\textcolor{CrossRed}{0.8716 {\scriptsize\(\pm \ 0.0045\)}}} &
\textbf{\textcolor{CrossRed}{0.6663 {\scriptsize\(\pm \ 0.0047\)}}} &
\textbf{\textcolor{CrossRed}{0.6230 {\scriptsize\(\pm \ 0.0029\)}}} &
\textbf{\textcolor{CrossRed}{0.6191 {\scriptsize\(\pm \ 0.0026\)}}} &
\textbf{\textcolor{CrossRed}{0.6357 {\scriptsize\(\pm \ 0.0047\)}}} &
\textbf{\textcolor{CrossRed}{0.6335 {\scriptsize\(\pm \ 0.0041\)}}} &
\textbf{\textcolor{CrossRed}{0.6332 {\scriptsize\(\pm \ 0.0044\)}}} \\ \cmidrule(lr){2-11}

 &
\textit{\textbf{Nepco \textbf{\textcolor{CheckBlue}{\ding{51}}}}} &
\textbf{\uline{0.8897 {\scriptsize\(\pm \ 0.0074\)}}} &
\textbf{\uline{0.8747 {\scriptsize\(\pm \ 0.0035\)}}} &
\textbf{\uline{0.8719 {\scriptsize\(\pm \ 0.0027\)}}} &
\textbf{\uline{0.6752 {\scriptsize\(\pm \ 0.0044\)}}} &
\textbf{\uline{0.6499 {\scriptsize\(\pm \ 0.0032\)}}} &
\textbf{\uline{0.6457 {\scriptsize\(\pm \ 0.0033\)}}} &
\textbf{\uline{0.6413 {\scriptsize\(\pm \ 0.0040\)}}} &
\textbf{\uline{0.6306 {\scriptsize\(\pm \ 0.0029\)}}} &
\textbf{\uline{0.6316 {\scriptsize\(\pm \ 0.0030\)}}} \\

\bottomrule

\multicolumn{11}{l}{\textsuperscript{1} We consider the early-stage analysis setting using the first 5 packets of each flow, which represents a constrained-setting comparison for hardware-offloadable models with longer observations.} \\

\end{tabular}%
}
\vspace{-12pt}
\end{table*}



\cg{We further evaluate \textit{Nepco} and baselines on three more network traffic datasets, i.e., CSTNET-20, CSTNET-120, and DoHBrw, which are adopted in recent network foundation model studies \cite{TrafficFormer-SP25,TrafficLLM-arXiv25}.
CSTNET-20 and CSTNET-120 are derived from the publicly available CSTNET-TLS1.3 \cite{ET-BERT-WWW22} dataset, which contains TLS 1.3-encrypted traffic from 120 mobile application classes.
Following the dataset settings of recent work, we use the complete dataset as CSTNET-120, and construct CSTNET-20 using the 20-class split released in the TrafficLLM repository \cite{TrafficLLM-arXiv25}.
DoHBrw \cite{DoHBrw-DASC20} contains four benign DNS-over-HTTPS (DoH) classes and one malicious DoH class.
Following the 5-class setting in TrafficLLM, we use it for the malicious DoH classification task.}

\cg{As shown in TABLE~\ref{tab:Additional Classification Performance}, \textit{Nepco} achieves competitive classification performance with existing network foundation models across the three network traffic datasets.
On CSTNET-20 and CSTNET-120, \textit{Nepco} achieves macro F1 scores of 0.8719 and 0.6457, improving upon the highest macro F1 scores achieved by existing network foundation models by 0.03\% and 4.30\%, respectively.
On DoHBrw, \textit{Nepco} achieves a macro F1 of 0.6316, which is 0.25\% lower than TrafficFormer’s 0.6332, the highest macro F1 among existing network foundation models.
Under the constrained early-stage analysis setting, \textit{Nepco} also consistently outperforms existing hardware-offloadable models across the three more datasets, improving macro F1 over Flowrest, Leo, Mousika, and BoS by 63.23\%, 695.72\%, 109.44\%, and 504.95\% on average, respectively.}
