# Supplementary material for: Versatile yet Efficient Network Traffic Analysis: Offloading Network Foundation Model to SmartNIC
Source: arXiv:2508.02001 source file (2026-11-12)
Supplement: Supplementary file 5 [file Support.tex]

\section{Supporting Materials}
\label{app:Supporting Materials}

Due to space limitations, detailed analyses and additional experiments are provided in our supporting materials \cite{Nepco-Appendix}.

\subsection{The Impact of Address-related Information}

\label{Address}

Since existing network foundation models follow the pre-training and fine-tuning paradigm, we examine the impact of address-related information across these two stages and make two experimental observations:


\begin{enumerate}
    \item In the pre-training stage, introducing address-related pre-training tasks leads to substantial inflation in downstream classification performance.
    
    \item In the fine-tuning stage, retaining address-related information yields spurious classification performance gains that do not survive simple protocol field randomization.
    
\end{enumerate}




In the pre-training stage, Pcap-Encoder \cite{Pcap-Encoder-SIGCOMM25} is the only network foundation model (to the best of our knowledge) that explicitly incorporates address-related information into its pre-training tasks, e.g., predicting the IP source/destination addresses of packets.
We pre-train two variants of Pcap-Encoder—with and without these tasks—and evaluate them on six traffic analysis tasks.
As shown in Fig. \ref{fig:Address-Pretraining}, removing them causes an average macro F1 drop of 34.69\%, e.g., from 0.9008 to 0.5020 on ISCX-VPN-Service.
This also explains Pcap-Encoder's lower performance in TABLE \ref{tab:Overall Classification Performance}, where all baselines are evaluated under our unbiased setting.




In the fine-tuning stage, we evaluate four network foundation models—NetGPT, ET-BERT, TraGe, and TrafficFormer—as TABLE \ref{tab:Overall Classification Performance} shows that they achieve markedly higher classification performance than other models.
We consider three settings: (i) zeroing out address-related fields in both training and test sets, (ii) retaining address-related fields in both, and (iii) retaining address-related fields in training but randomizing them in the test set.
As shown in Fig. \ref{fig:Address-Finetuning}, retaining address fields inflates macro F1 by 5.19\% on average over zeroing them out, but once test-time address fields are randomized, macro F1 drops by 44.67\% on average.
This sharp degradation indicates that the gains from retaining address fields stem from shortcut learning on address-related cues rather than from learning transferable traffic semantics.
Therefore, we zero out address-related protocol fields during traffic processing to ensure that the model learns transferable traffic semantics rather than address-related shortcuts, thereby providing unbiased estimates of generalization.
% Therefore, we zero out address-related fields to ensure unbiased generalization estimates.


% In the fine-tuning stage, we evaluate four network foundation models—NetGPT, ET-BERT, TraGe, and TrafficFormer—which achieve markedly higher performance than other models in TABLE~\ref{tab:Overall Classification Performance}.
% We consider three settings: (i) zeroing out address-related fields in both training and test sets, (ii) retaining them in both, and (iii) retaining them in training but randomizing them at test time.
% As shown in Fig.~\ref{fig:Address-Finetuning}, retaining address fields inflates macro F1 by 5.19\% on average over zeroing them out, but once test-time address fields are randomized, macro F1 drops by 44.67\% on average.
% This degradation indicates that the gains stem from shortcut learning on address-related cues rather than from transferable traffic semantics



% \clearpage

\subsection{Cross-Dataset Localized Byte-sequence Pattern}

\label{Local-Pattern}

We further examine localized byte-sequence patterns across datasets through quantitative analysis, providing additional support for the four observations in Section \ref{sec:Localized Pattern-Aware Traffic Modeling}.
As conducting this analysis on every public dataset is infeasible, we select two representative datasets, i.e., USTC-TFC, which is part of our fine-tuning evaluation, and CIC-IoT, which is held out from both pre-training and fine-tuning, covering both in-evaluation and out-of-evaluation settings.
We present four observation supports (\textbf{OS1–OS4}), each providing quantitative analysis for the corresponding observation (\textbf{O1–O4}).

\begin{figure}[t]
  \centering
  \includegraphics[width=0.8\linewidth]{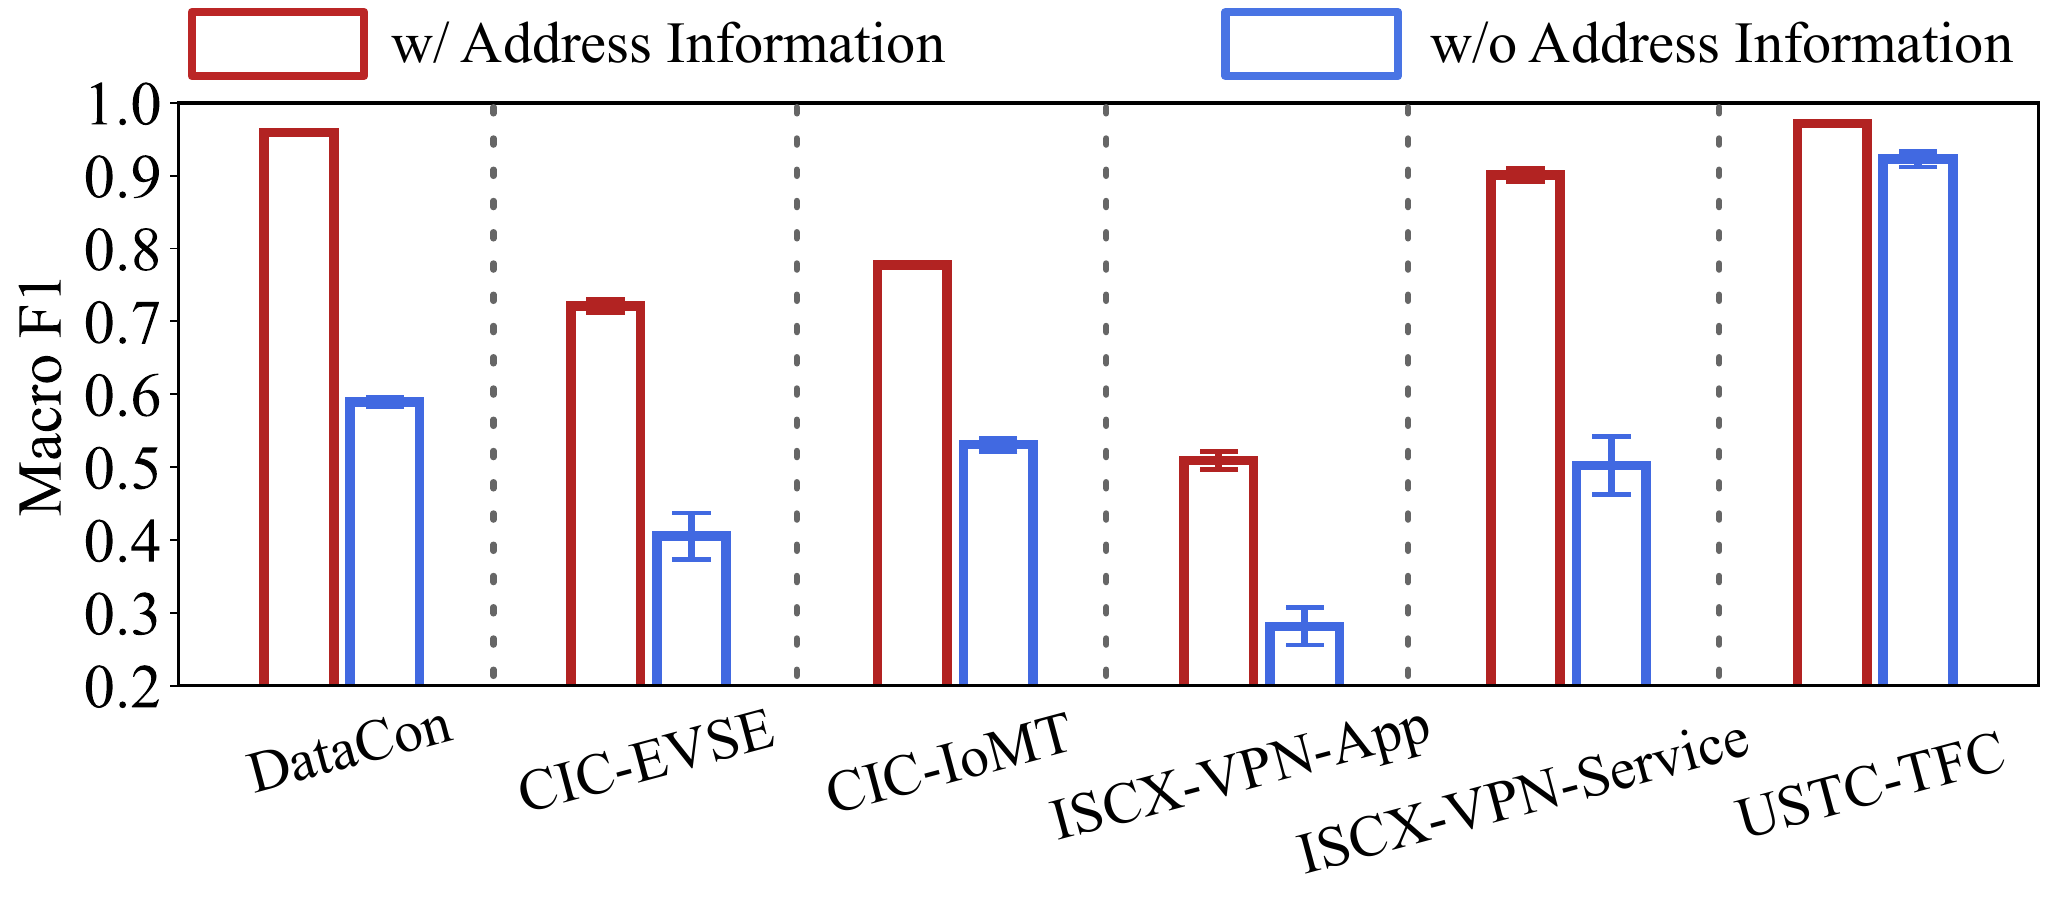}
  \caption{Impact of address-related pre-training tasks on Pcap-Encoder's performance across six traffic analysis tasks.}
  \vspace{-12pt}
  \label{fig:Address-Pretraining}
\end{figure}

\begin{figure*}[t]
  \centering
  \includegraphics[width=\linewidth]{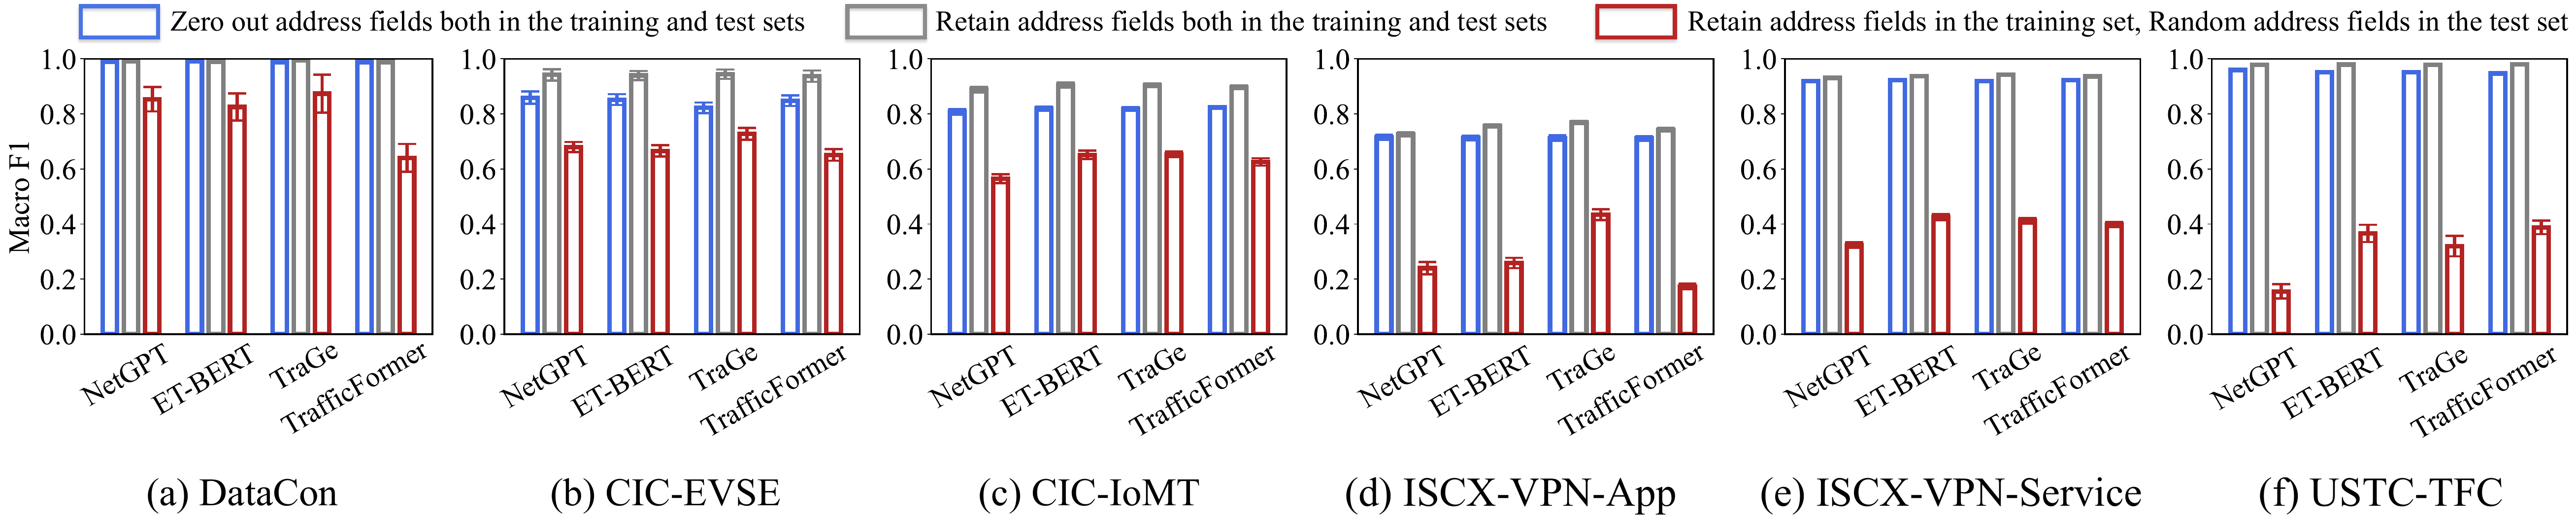}
  \caption{Impact of address-related information during the fine-tuning stage across six network traffic analysis tasks.}
  \vspace{-12pt}
  \label{fig:Address-Finetuning}
\end{figure*}


\begin{figure}[t]
  \centering
  \includegraphics[width=1\linewidth]{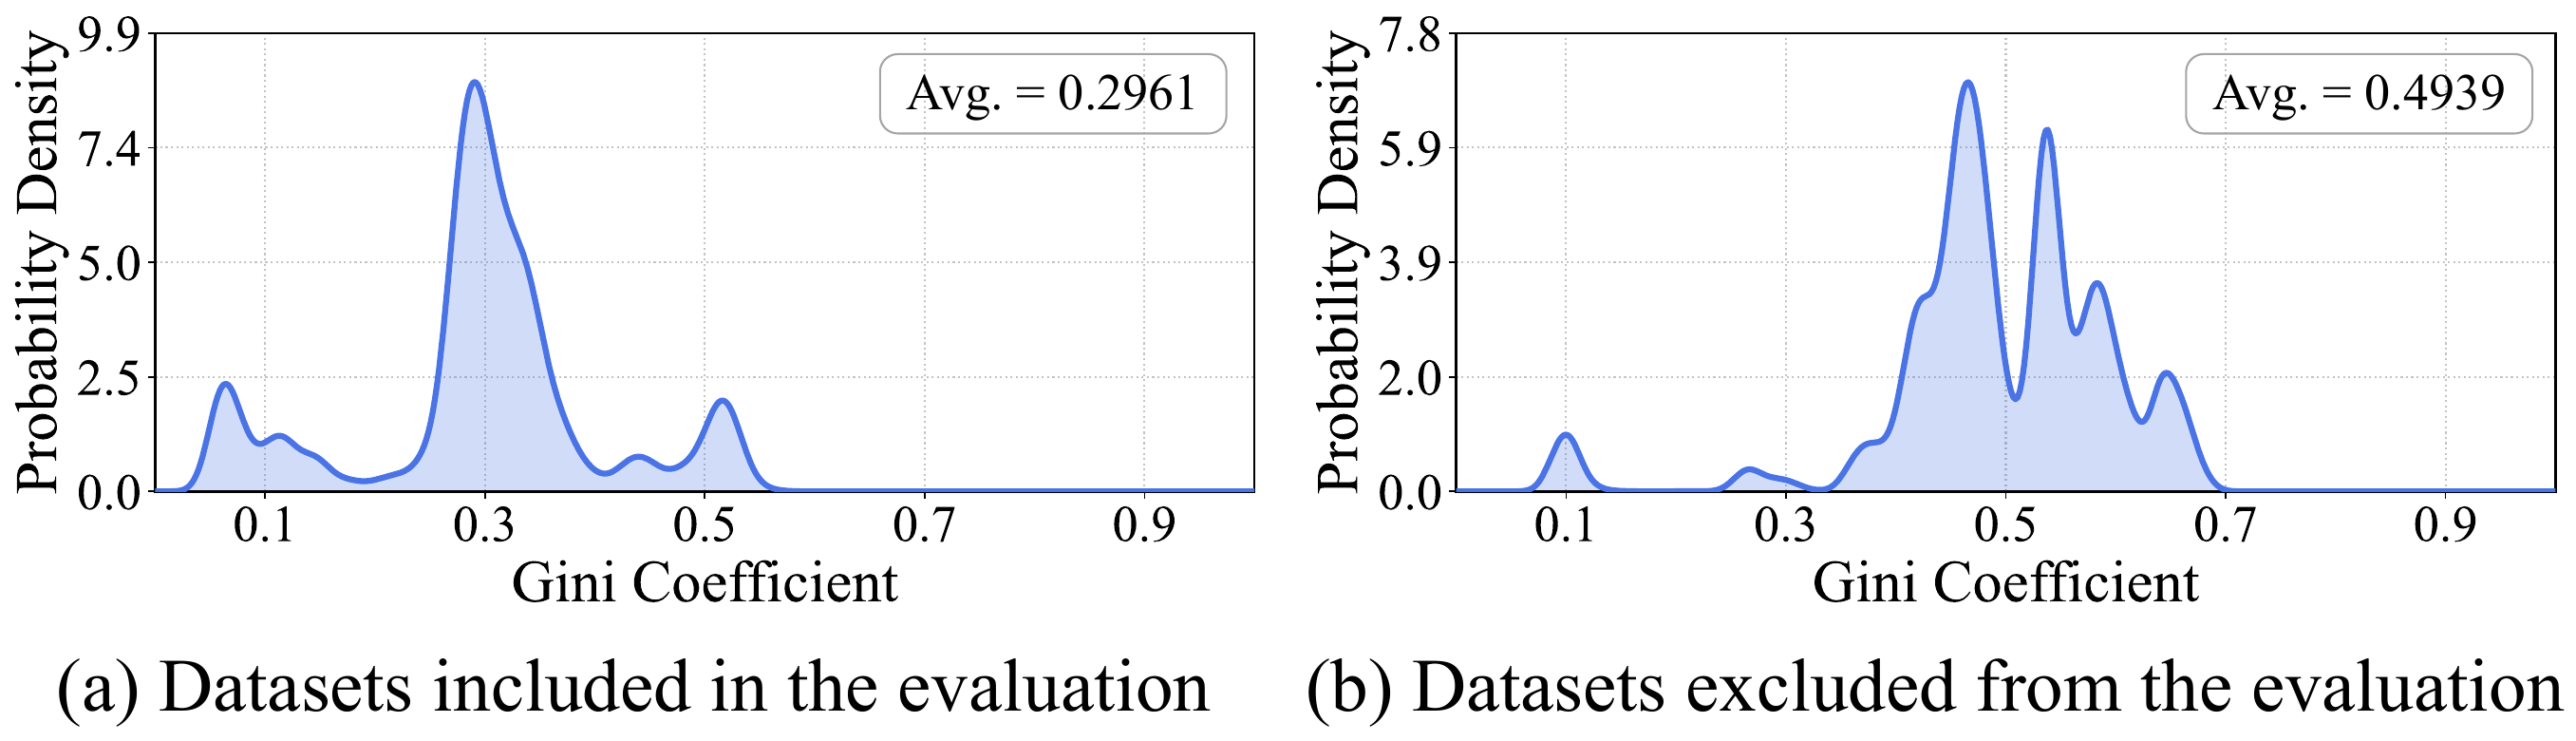}
  \caption{Distribution of Gini coefficients computed on byte importance score sequences.}
  \vspace{-10pt}
  \label{fig:Gini}
\end{figure}


\begin{figure}[t]
  \centering
  \includegraphics[width=1\linewidth]{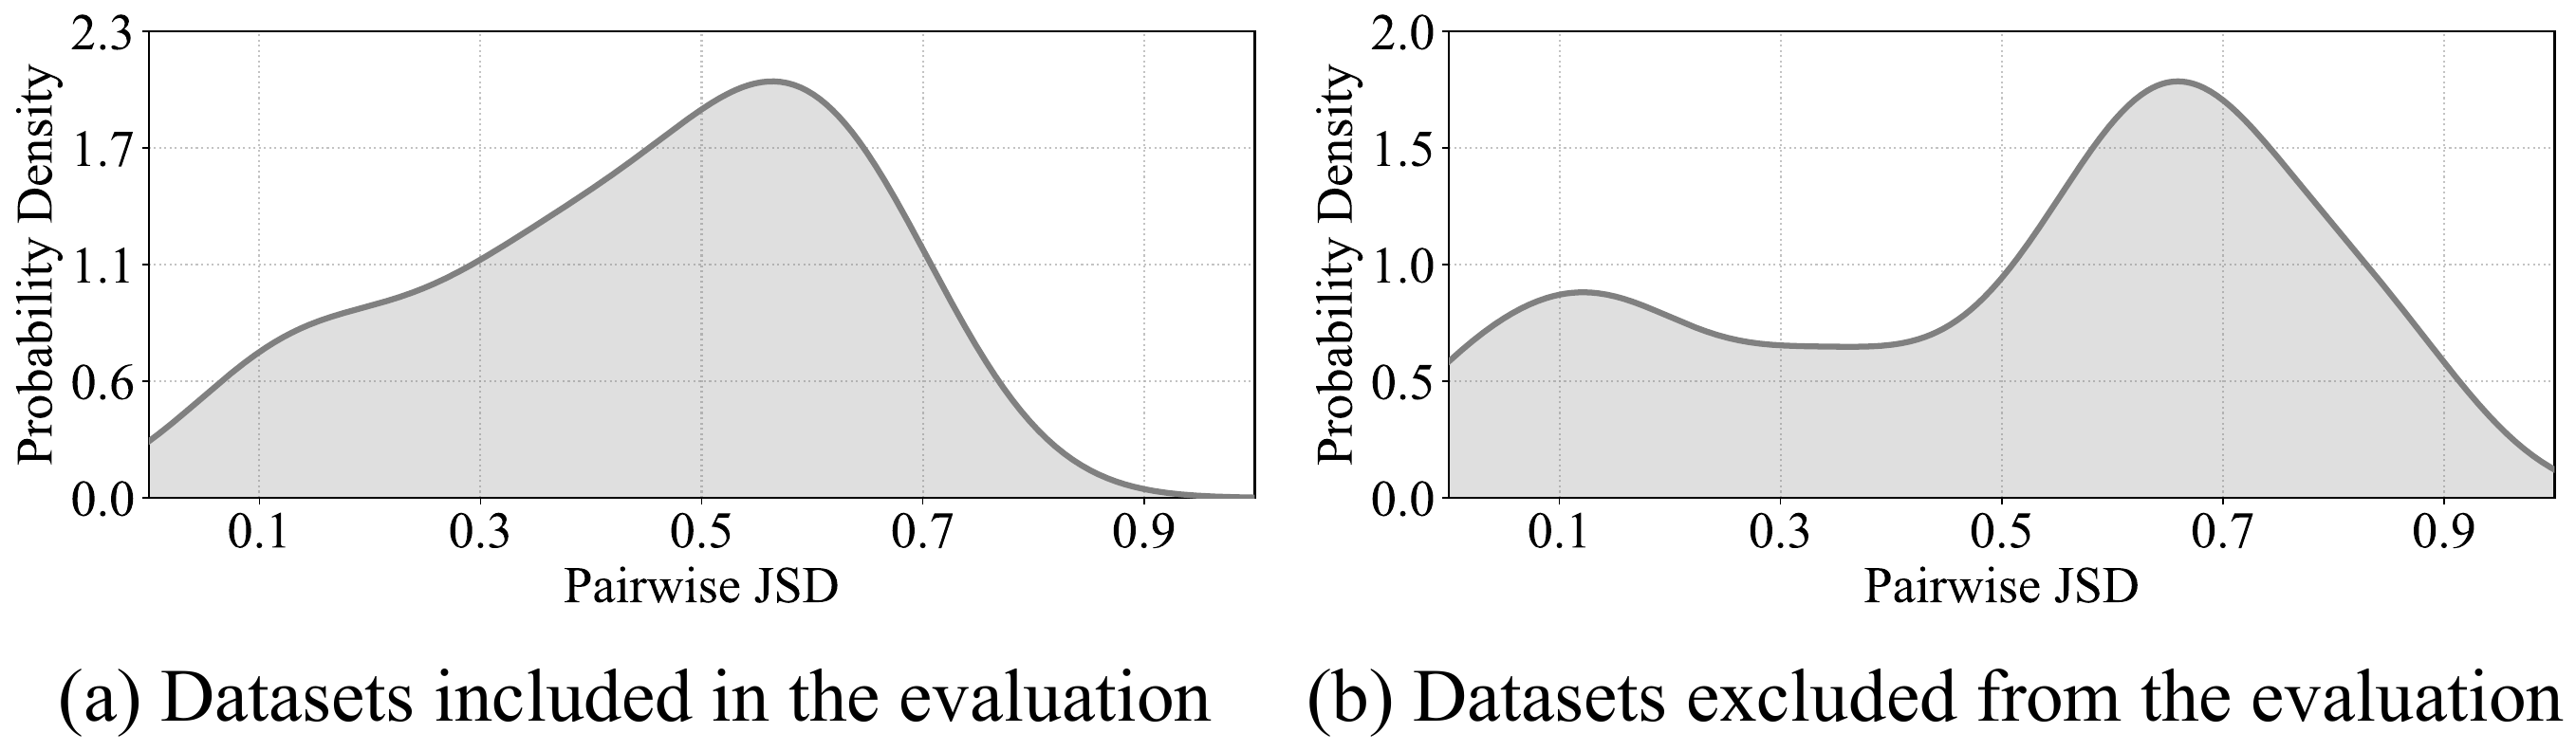}
  \caption{Distribution of pairwise Jensen-Shannon Divergence between per-class field distributions.}
  \vspace{-10pt}
  \label{fig:Pair-JSD}
\end{figure}

% \vspace{0.05in}
\noindent\textbf{\cg{OS1: Discriminative traffic patterns are often localized.}}
% We compute the Gini coefficient \cite{Gini} of the byte importance score sequences, which quantifies how unevenly the importance is distributed: a value close to 0 means importance is spread across all bytes, while a value close to 1 means a few bytes hold most of the importance.
% In Fig.~\ref{fig:Gini}, the per-packet Gini is centered above zero on both datasets (Fig.~\ref{fig:Gini}(a), averaging 0.2961; Fig.~\ref{fig:Gini}(b), averaging 0.4939), indicating that byte importance is concentrated on a small subset of positions.
We compute the Gini coefficient \cite{Gini} of the byte importance score sequences to quantify how unevenly importance is distributed across byte positions.
A value close to 0 indicates uniform distribution, while a value close to 1 indicates concentration on a few bytes.
As shown in Fig.~\ref{fig:Gini}, the Gini distributions are right-skewed and consistently centered above zero on both datasets, averaging 0.2961 on USTC-TFC (Fig.~\ref{fig:Gini}(a)) and 0.4939 on CIC-IoT (Fig.~\ref{fig:Gini}(b)).
% The right-skewed shape indicates that the majority of traffic samples exhibit meaningful locality rather than a small fraction of outliers driving the average upward, confirming that byte importance concentration is a general property of network traffic rather than an artifact of any particular dataset.
\cg{This distribution provides evidence that byte importance is non-uniform and often concentrated on subsets of byte positions rather than being uniformly distributed across the sequence. This provides cross-dataset support for the locality observation, suggesting that it is not limited to a single evaluation dataset.}


% \vspace{0.05in}
\noindent\textbf{\cg{OS2: Different categories favor different local regions.}}
% For each packet, we identify its Top-5 most important protocol fields and aggregate per-class field distributions.
% We then compute the pairwise Jensen-Shannon Divergence (JSD) \cite{JSD} between every pair of classes, where a higher JSD indicates more divergent field preferences.
% In Fig.~\ref{fig:Pair-JSD}, the pairwise JSD is above zero on both datasets, indicating that distinct classes rely on substantially different sets of protocol fields.
For each traffic sample, we identify its Top-5 most important protocol fields and aggregate the field-level importance distribution per class.
We then compute the pairwise Jensen-Shannon Divergence (JSD) \cite{JSD} between per-class distributions for every pair of classes, where a higher JSD indicates more divergent field preferences.
As shown in Fig.~\ref{fig:Pair-JSD}, the pairwise JSD distribution is consistently above zero across all class pairs on both datasets, with the bulk of mass concentrated at moderate-to-high divergence values. 
% This confirms that distinct traffic classes concentrate their importance on substantially different protocol field regions, validating that localized modeling retains sufficient discriminative capacity for multi-class analysis.
\cg{This provides evidence that different traffic classes may rely on discriminative information located in different field regions.}

% \vspace{0.05in}
\noindent\textbf{\cg{OS3: Discriminative bytes often occupy only part of a field.}}
% For each packet, we identify the protocol fields hit by its Top-5 most important bytes, and compute the Gini coefficient on the byte importance score sequence within each hit field.
% As shown in Fig.~\ref{fig:Gini-Field}, the field-level Gini is above zero on both datasets (Fig.~\ref{fig:Gini-Field}(a), averaging 0.2907; Fig.~\ref{fig:Gini-Field}(b), averaging 0.4389), indicating that even within high-importance fields, only a subset of bytes is highly weighted.
For each traffic sample, we identify the protocol fields hit by its Top-5 most important bytes and compute the Gini coefficient over the byte importance scores within each such field.
As shown in Fig.~\ref{fig:Gini-Field}, the field-level Gini is consistently above zero on both datasets, averaging 0.2907 on USTC-TFC (Fig.~\ref{fig:Gini-Field}(a)) and 0.4389 on CIC-IoT (Fig.~\ref{fig:Gini-Field}(b)), indicating that even within high-importance protocol fields, only a subset of bytes is highly weighted.
% This intra-field selectivity motivates the window-wise byte scoring in \textit{Nepco}, which assigns learnable per-position weights within each convolution window rather than treating all bytes uniformly.



% \vspace{0.05in}
\noindent\textbf{OS4: Address fields attract disproportionate importance.}
% For each packet, we measure how often each of the eight address-related fields is hit by its Top-5 most important bytes, and report the \textit{At-Least-One Hit@5} metric—the fraction of packets in which at least one address-related field is hit.
% As shown in Fig.~\ref{fig:Address_Hit}, the metric reaches 0.8816 on Fig.~\ref{fig:Address_Hit}(a) and 0.9675 on Fig.~\ref{fig:Address_Hit}(b), indicating that without address zeroing, the model's importance is dominated by address-related fields.
For each traffic sample, we measure how often each of the eight address-related protocol fields is hit by its Top-5 most important bytes, and report the At-Least-One Hit@5 metric, defined as the fraction of traffic samples in which at least one address-related field is hit.
As shown in Fig.~\ref{fig:Address_Hit}, the metric reaches 0.8816 on USTC-TFC (Fig.~\ref{fig:Address_Hit}(a)) and 0.9675 on CIC-IoT (Fig.~\ref{fig:Address_Hit}(b)), indicating that without address zeroing, address-related fields dominate byte importance in the vast majority of traffic samples. Since these fields carry no transferable traffic semantics, this confirms that address zeroing is necessary not only for evaluation validity but also to redirect the model toward learning class-discriminative traffic patterns.


\begin{figure}[t]
  \centering
  \includegraphics[width=1\linewidth]{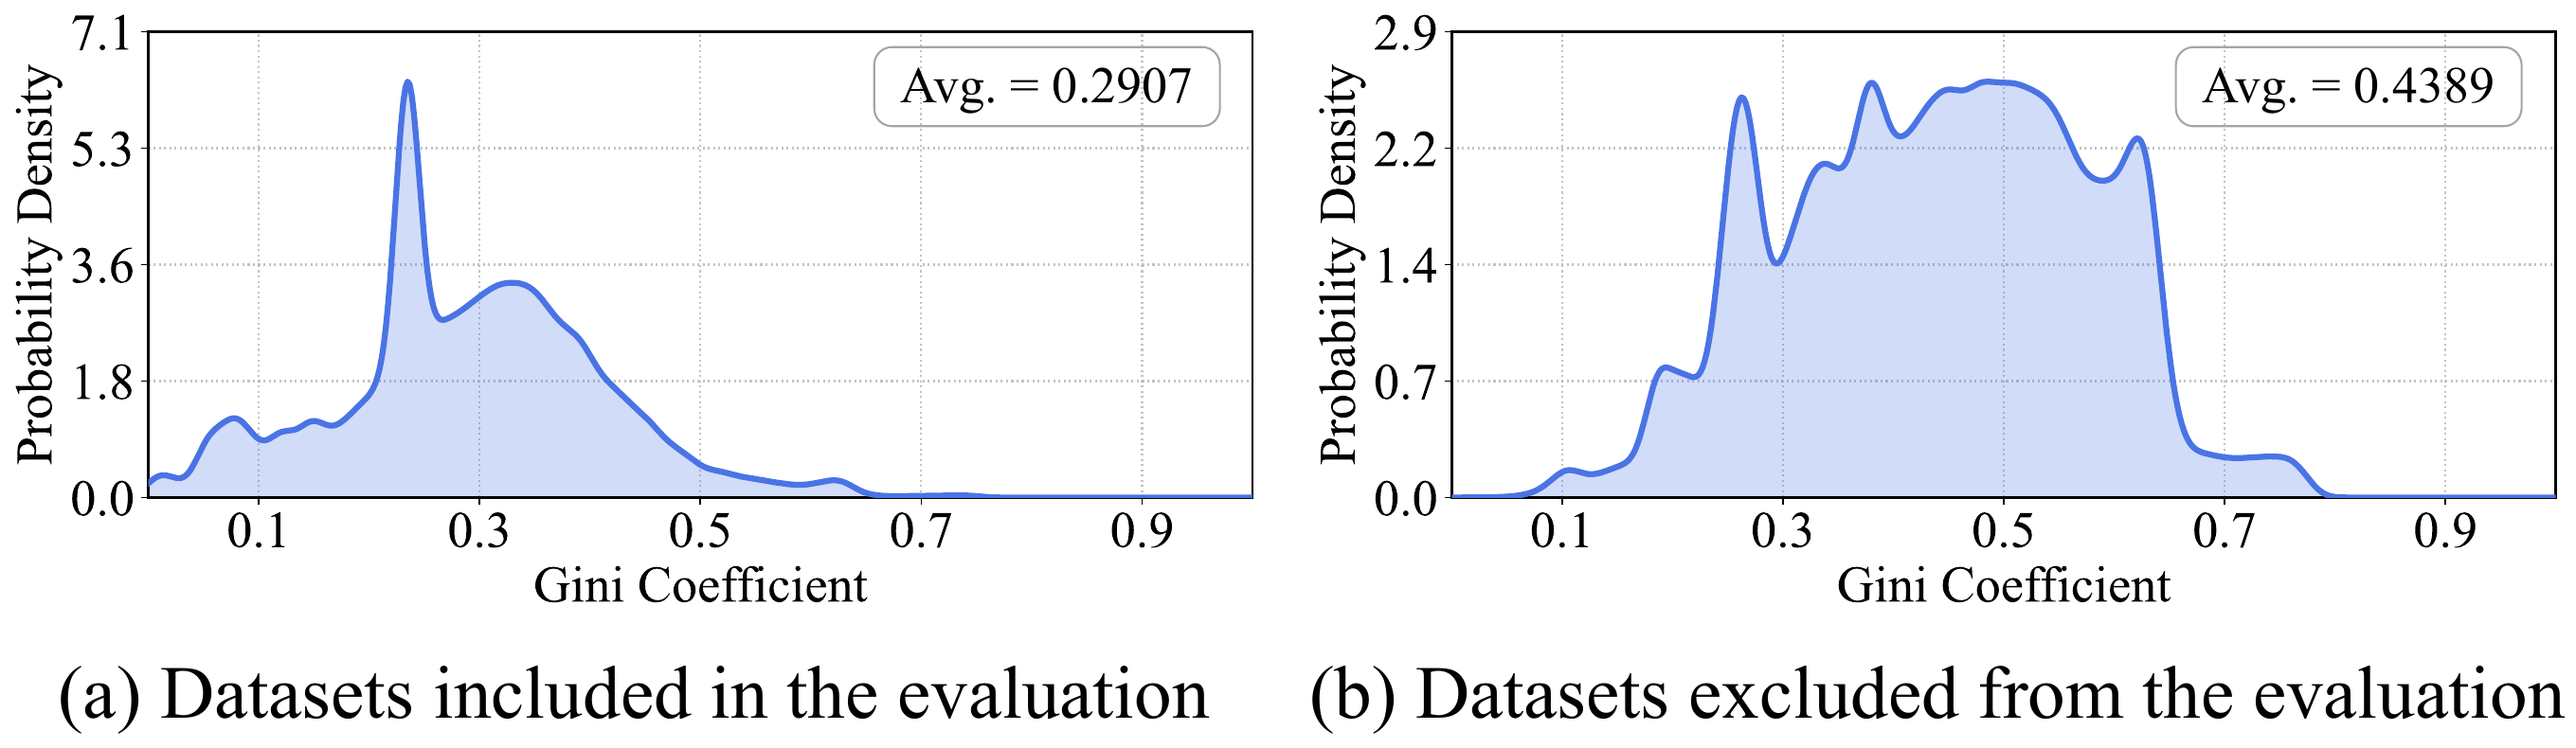}
  \caption{Distribution of per-sequence Gini coefficients of byte importance scores within each Top-5 protocol field.}
  \vspace{-10pt}
  \label{fig:Gini-Field}
\end{figure}



\begin{figure}[t]
  \centering
  \includegraphics[width=1\linewidth]{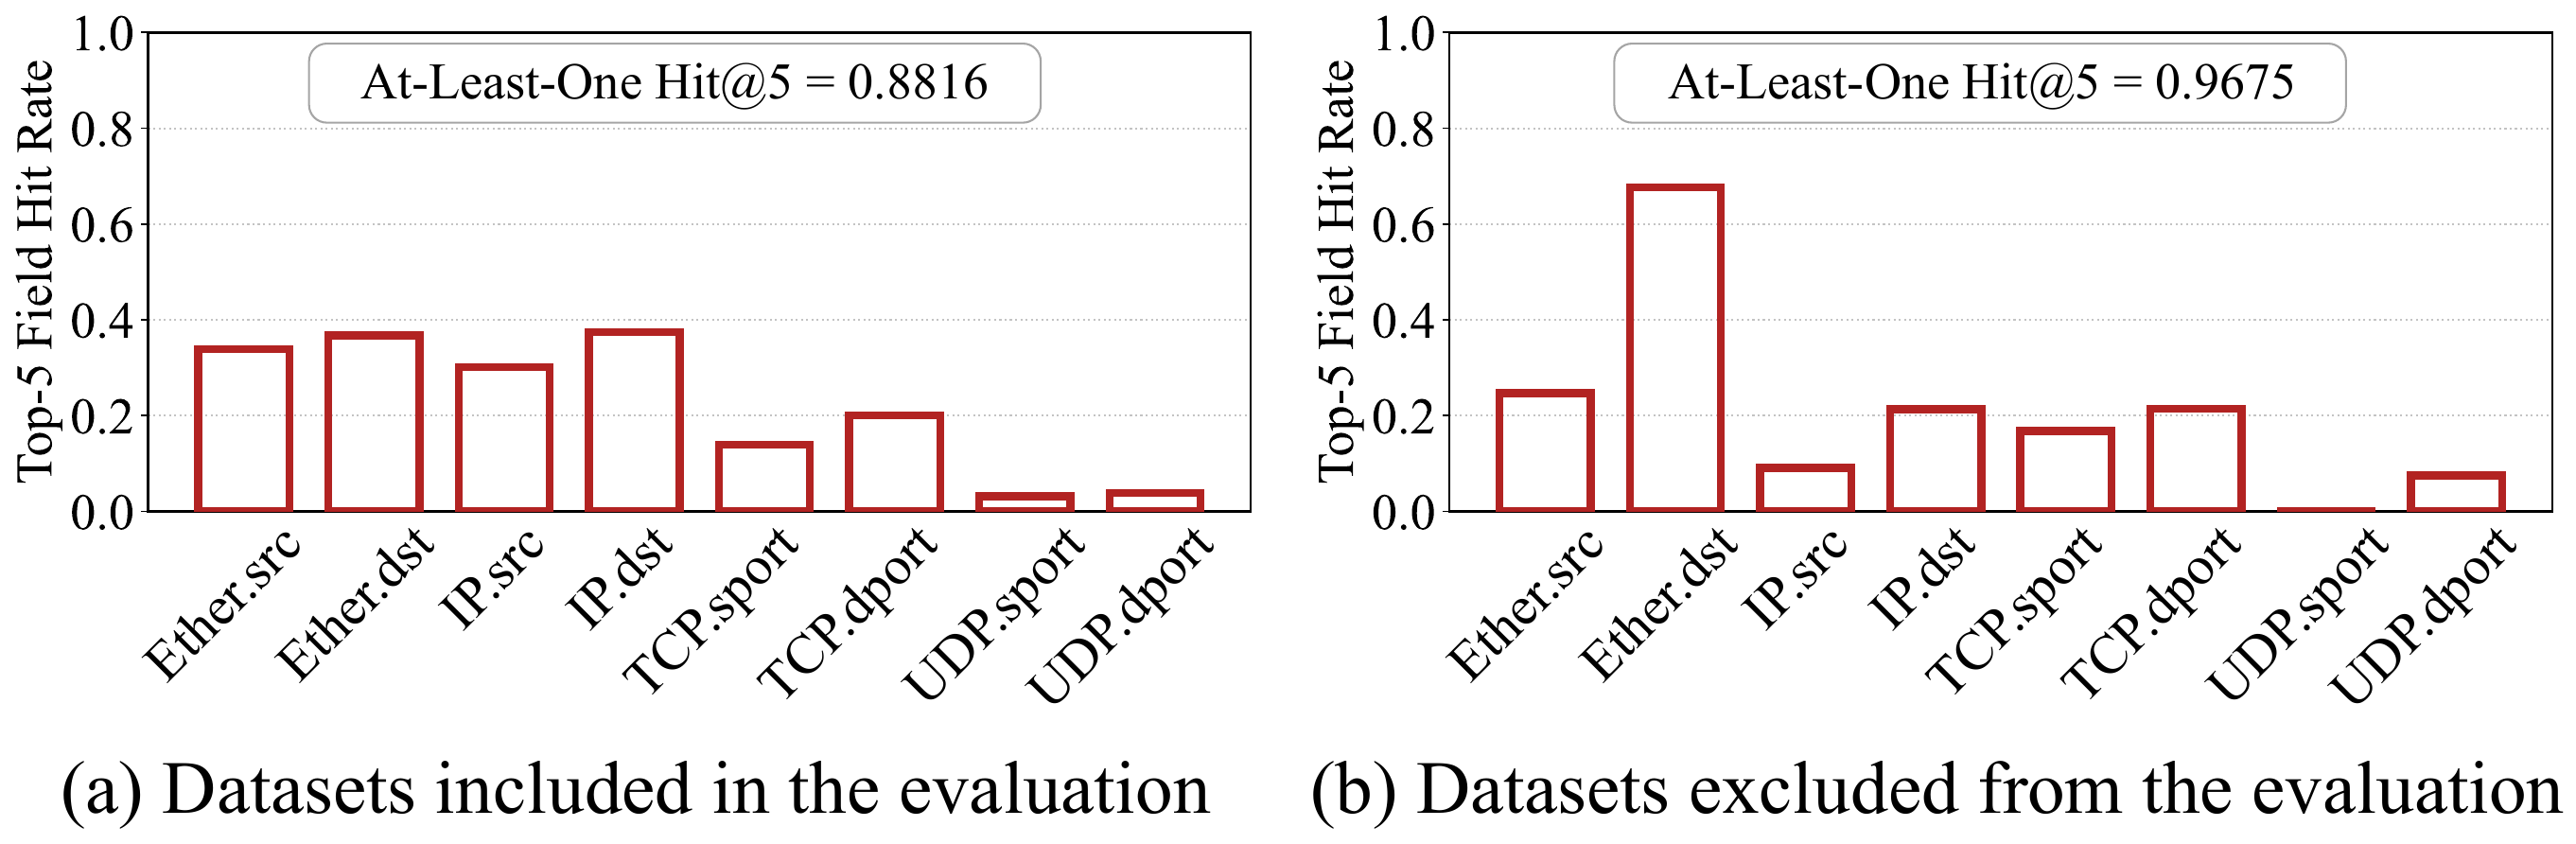}
  \caption{Hit frequency of eight address-related protocol fields in the Top-5 most important bytes.}
  \vspace{-10pt}
  \label{fig:Address_Hit}
\end{figure}


\subsection{\cg{Evaluation on Three More Network Traffic Datasets}}

\label{New_Dataset}

\begin{table*}[t!]
\renewcommand{\arraystretch}{1.1}
\centering
\small
\caption{\cg{The overall classification performances of \textit{Nepco} and baselines on three more network traffic datasets.}}
\label{tab:Additional Classification Performance}
\resizebox{1\textwidth}{!}{%
\begin{tabular}{c|c|ccc|ccc|ccc}

\toprule
\multicolumn{2}{c|}{\multirow{2}{*}{\textbf{Method} \textsuperscript{1}}} &
\multicolumn{3}{c|}{\textbf{CSTNET-20 (2023)}} &
\multicolumn{3}{c|}{\textbf{CSTNET-120 (2023)}} &
\multicolumn{3}{c}{\textbf{DoHBrw (2020)}} \\

\multicolumn{2}{c|}{} &
Precision &
Recall &
Macro F1 &
Precision &
Recall &
Macro F1 &
Precision &
Recall &
Macro F1 \\ \midrule

\multirow{9}{*}{\rotatebox[origin=c]{90}{\makecell{ML/DL Model \\ \textbf{\textcolor{CheckBlue}{\ding{51}}}: Hardware-Offloadable}}} &
FlowPrint &
0.0992 {\scriptsize\(\pm \ 0.0110\)} &
0.1314 {\scriptsize\(\pm \ 0.0124\)} &
0.0971 {\scriptsize\(\pm \ 0.0108\)} &
0.0953 {\scriptsize\(\pm \ 0.0043\)} &
0.1023 {\scriptsize\(\pm \ 0.0025\)} &
0.0850 {\scriptsize\(\pm \ 0.0027\)} &
0.2843 {\scriptsize\(\pm \ 0.0244\)} &
0.3120 {\scriptsize\(\pm \ 0.0195\)} &
0.2853 {\scriptsize\(\pm \ 0.0213\)} \\

 &
AppScanner &
0.6962 {\scriptsize\(\pm \ 0.0024\)} &
0.6809 {\scriptsize\(\pm \ 0.0024\)} &
0.6825 {\scriptsize\(\pm \ 0.0024\)} &
0.5571 {\scriptsize\(\pm \ 0.0018\)} &
0.5002 {\scriptsize\(\pm \ 0.0012\)} &
0.5148 {\scriptsize\(\pm \ 0.0012\)} &
0.4749 {\scriptsize\(\pm \ 0.0015\)} &
0.4586 {\scriptsize\(\pm \ 0.0016\)} &
0.4560 {\scriptsize\(\pm \ 0.0014\)} \\

 &
XGBoost &
0.6921 {\scriptsize\(\pm \ 0.0248\)} &
0.6637 {\scriptsize\(\pm \ 0.0329\)} &
0.6795 {\scriptsize\(\pm \ 0.0214\)} &
0.2985 {\scriptsize\(\pm \ 0.0185\)} &
0.2851 {\scriptsize\(\pm \ 0.0164\)} &
0.2818 {\scriptsize\(\pm \ 0.0183\)} &
0.4652 {\scriptsize\(\pm \ 0.0114\)} &
0.4367 {\scriptsize\(\pm \ 0.0157\)} &
0.4412 {\scriptsize\(\pm \ 0.0148\)} \\

 &
DTree &
0.5628 {\scriptsize\(\pm \ 0.0341\)} &
0.5324 {\scriptsize\(\pm \ 0.0413\)} &
0.5515 {\scriptsize\(\pm \ 0.0409\)} &
0.2124 {\scriptsize\(\pm \ 0.0103\)} &
0.2021 {\scriptsize\(\pm \ 0.0198\)} &
0.2097 {\scriptsize\(\pm \ 0.0125\)} &
0.4113 {\scriptsize\(\pm \ 0.0123\)} &
0.4067 {\scriptsize\(\pm \ 0.0196\)} &
0.4119 {\scriptsize\(\pm \ 0.0187\)} \\

 &
Flowrest \textbf{\textcolor{CheckBlue}{\ding{51}}} &
\textbf{\textcolor{CheckBlue}{\uline{0.7161 {\scriptsize\(\pm \ 0.0142\)}}}} &
\textbf{\textcolor{CheckBlue}{\uline{0.6857 {\scriptsize\(\pm \ 0.0081\)}}}} &
\textbf{\textcolor{CheckBlue}{\uline{0.6803 {\scriptsize\(\pm \ 0.0098\)}}}} &
0.3297 {\scriptsize\(\pm \ 0.0099\)} &
\textbf{\textcolor{CheckBlue}{\uline{0.2980 {\scriptsize\(\pm \ 0.0043\)}}}} &
\textbf{\textcolor{CheckBlue}{\uline{0.2659 {\scriptsize\(\pm \ 0.0054\)}}}} &
\textbf{\textcolor{CheckBlue}{\uline{0.5354 {\scriptsize\(\pm \ 0.0032\)}}}} &
\textbf{\textcolor{CheckBlue}{\uline{0.5367 {\scriptsize\(\pm \ 0.0039\)}}}} &
\textbf{\textcolor{CheckBlue}{\uline{0.5322 {\scriptsize\(\pm \ 0.0040\)}}}} \\

 &
Leo \textbf{\textcolor{CheckBlue}{\ding{51}}} &
0.2986 {\scriptsize\(\pm \ 0.0106\)} &
0.3901 {\scriptsize\(\pm \ 0.0055\)} &
0.3142 {\scriptsize\(\pm \ 0.0074\)} &
0.0211 {\scriptsize\(\pm \ 0.0003\)} &
0.0993 {\scriptsize\(\pm \ 0.0010\)} &
0.0330 {\scriptsize\(\pm \ 0.0004\)} &
0.4412 {\scriptsize\(\pm \ 0.0215\)} &
0.4470 {\scriptsize\(\pm \ 0.0053\)} &
0.4128 {\scriptsize\(\pm \ 0.0085\)} \\

 &
Mousika \textbf{\textcolor{CheckBlue}{\ding{51}}} &
0.6151 {\scriptsize\(\pm \ 0.0202\)} &
0.4896 {\scriptsize\(\pm \ 0.0086\)} &
0.4725 {\scriptsize\(\pm \ 0.0107\)} &
\textbf{\textcolor{CheckBlue}{\uline{0.3752 {\scriptsize\(\pm \ 0.0062\)}}}} &
0.2580 {\scriptsize\(\pm \ 0.0020\)} &
0.2412 {\scriptsize\(\pm \ 0.0019\)} &
0.3922 {\scriptsize\(\pm \ 0.0372\)} &
0.4403 {\scriptsize\(\pm \ 0.0025\)} &
0.3587 {\scriptsize\(\pm \ 0.0018\)} \\

 &
EBSNN &
0.8234 {\scriptsize\(\pm \ 0.0404\)} &
0.7915 {\scriptsize\(\pm \ 0.0438\)} &
0.7819 {\scriptsize\(\pm \ 0.0475\)} &
0.6052 {\scriptsize\(\pm \ 0.0274\)} &
0.5600 {\scriptsize\(\pm \ 0.0256\)} &
0.5426 {\scriptsize\(\pm \ 0.0281\)} &
0.5354 {\scriptsize\(\pm \ 0.0302\)} &
0.5139 {\scriptsize\(\pm \ 0.0178\)} &
0.4897 {\scriptsize\(\pm \ 0.0277\)} \\

 &
BoS \textbf{\textcolor{CheckBlue}{\ding{51}}} &
0.3370 {\scriptsize\(\pm \ 0.0136\)} &
0.3795 {\scriptsize\(\pm \ 0.0167\)} &
0.3815 {\scriptsize\(\pm \ 0.0125\)} &
0.0183 {\scriptsize\(\pm \ 0.0012\)} &
0.0175 {\scriptsize\(\pm \ 0.0018\)} &
0.0446 {\scriptsize\(\pm \ 0.0023\)} &
0.4103 {\scriptsize\(\pm \ 0.0070\)} &
0.4113 {\scriptsize\(\pm \ 0.0158\)} &
0.4559 {\scriptsize\(\pm \ 0.0038\)} \\

\midrule

\multirow{9}{*}{\rotatebox[origin=c]{90}{\makecell{Network Foundation Model \\ \textbf{\textcolor{CheckBlue}{\ding{51}}}: Hardware-Offloadable}}} &
NetMamba &
0.8672 {\scriptsize\(\pm \ 0.0104\)} &
0.8393 {\scriptsize\(\pm \ 0.0093\)} &
0.8435 {\scriptsize\(\pm \ 0.0100\)} &
0.4246 {\scriptsize\(\pm \ 0.0735\)} &
0.4256 {\scriptsize\(\pm \ 0.0742\)} &
0.3947 {\scriptsize\(\pm \ 0.0689\)} &
0.5474 {\scriptsize\(\pm \ 0.0077\)} &
0.5380 {\scriptsize\(\pm \ 0.0056\)} &
0.5316 {\scriptsize\(\pm \ 0.0051\)} \\

 &
YaTC &
0.8293 {\scriptsize\(\pm \ 0.0054\)} &
0.8309 {\scriptsize\(\pm \ 0.0056\)} &
0.8122 {\scriptsize\(\pm \ 0.0056\)} &
0.6013 {\scriptsize\(\pm \ 0.0057\)} &
0.5834 {\scriptsize\(\pm \ 0.0039\)} &
0.5621 {\scriptsize\(\pm \ 0.0044\)} &
0.5516 {\scriptsize\(\pm \ 0.0051\)} &
0.5394 {\scriptsize\(\pm \ 0.0050\)} &
0.5398 {\scriptsize\(\pm \ 0.0052\)} \\

 &
Pcap-Encoder &
0.7417 {\scriptsize\(\pm \ 0.0152\)} &
0.7486 {\scriptsize\(\pm \ 0.0092\)} &
0.7370 {\scriptsize\(\pm \ 0.0110\)} &
0.3076 {\scriptsize\(\pm \ 0.0044\)} &
0.3909 {\scriptsize\(\pm \ 0.0034\)} &
0.3334 {\scriptsize\(\pm \ 0.0041\)} &
0.4770 {\scriptsize\(\pm \ 0.0044\)} &
0.4752 {\scriptsize\(\pm \ 0.0040\)} &
0.4737 {\scriptsize\(\pm \ 0.0042\)} \\

 &
PERT &
0.9001 {\scriptsize\(\pm \ 0.0090\)} &
0.8770 {\scriptsize\(\pm \ 0.0039\)} &
0.8703 {\scriptsize\(\pm \ 0.0050\)} &
0.6638 {\scriptsize\(\pm \ 0.0047\)} &
0.6151 {\scriptsize\(\pm \ 0.0025\)} &
0.6123 {\scriptsize\(\pm \ 0.0027\)} &
0.6258 {\scriptsize\(\pm \ 0.0057\)} &
0.6215 {\scriptsize\(\pm \ 0.0056\)} &
0.6213 {\scriptsize\(\pm \ 0.0056\)} \\

 &
NetGPT &
0.9025 {\scriptsize\(\pm \ 0.0064\)} &
0.8775 {\scriptsize\(\pm \ 0.0038\)} &
0.8702 {\scriptsize\(\pm \ 0.0041\)} &
0.6367 {\scriptsize\(\pm \ 0.0047\)} &
0.5934 {\scriptsize\(\pm \ 0.0034\)} &
0.5876 {\scriptsize\(\pm \ 0.0036\)} &
0.6167 {\scriptsize\(\pm \ 0.0046\)} &
0.6064 {\scriptsize\(\pm \ 0.0040\)} &
0.6060 {\scriptsize\(\pm \ 0.0037\)} \\

 &
ET-BERT &
0.9026 {\scriptsize\(\pm \ 0.0085\)} &
0.8788 {\scriptsize\(\pm \ 0.0041\)} &
0.8707 {\scriptsize\(\pm \ 0.0046\)} &
0.6562 {\scriptsize\(\pm \ 0.0044\)} &
0.6128 {\scriptsize\(\pm \ 0.0033\)} &
0.6082 {\scriptsize\(\pm \ 0.0036\)} &
0.6317 {\scriptsize\(\pm \ 0.0040\)} &
0.6274 {\scriptsize\(\pm \ 0.0038\)} &
0.6277 {\scriptsize\(\pm \ 0.0039\)} \\

 &
TraGe &
0.8823 {\scriptsize\(\pm \ 0.0064\)} &
0.8759 {\scriptsize\(\pm \ 0.0027\)} &
0.8674 {\scriptsize\(\pm \ 0.0035\)} &
0.6623 {\scriptsize\(\pm \ 0.0050\)} &
0.6189 {\scriptsize\(\pm \ 0.0025\)} &
0.6161 {\scriptsize\(\pm \ 0.0028\)} &
0.6319 {\scriptsize\(\pm \ 0.0066\)} &
0.6208 {\scriptsize\(\pm \ 0.0068\)} &
0.6220 {\scriptsize\(\pm \ 0.0074\)} \\

 &
TrafficFormer &
\textbf{\textcolor{CrossRed}{0.9033 {\scriptsize\(\pm \ 0.0070\)}}} &
\textbf{\textcolor{CrossRed}{0.8789 {\scriptsize\(\pm \ 0.0045\)}}} &
\textbf{\textcolor{CrossRed}{0.8716 {\scriptsize\(\pm \ 0.0045\)}}} &
\textbf{\textcolor{CrossRed}{0.6663 {\scriptsize\(\pm \ 0.0047\)}}} &
\textbf{\textcolor{CrossRed}{0.6230 {\scriptsize\(\pm \ 0.0029\)}}} &
\textbf{\textcolor{CrossRed}{0.6191 {\scriptsize\(\pm \ 0.0026\)}}} &
\textbf{\textcolor{CrossRed}{0.6357 {\scriptsize\(\pm \ 0.0047\)}}} &
\textbf{\textcolor{CrossRed}{0.6335 {\scriptsize\(\pm \ 0.0041\)}}} &
\textbf{\textcolor{CrossRed}{0.6332 {\scriptsize\(\pm \ 0.0044\)}}} \\ \cmidrule(lr){2-11}

 &
\textit{\textbf{Nepco \textbf{\textcolor{CheckBlue}{\ding{51}}}}} &
\textbf{\uline{0.8897 {\scriptsize\(\pm \ 0.0074\)}}} &
\textbf{\uline{0.8747 {\scriptsize\(\pm \ 0.0035\)}}} &
\textbf{\uline{0.8719 {\scriptsize\(\pm \ 0.0027\)}}} &
\textbf{\uline{0.6752 {\scriptsize\(\pm \ 0.0044\)}}} &
\textbf{\uline{0.6499 {\scriptsize\(\pm \ 0.0032\)}}} &
\textbf{\uline{0.6457 {\scriptsize\(\pm \ 0.0033\)}}} &
\textbf{\uline{0.6413 {\scriptsize\(\pm \ 0.0040\)}}} &
\textbf{\uline{0.6306 {\scriptsize\(\pm \ 0.0029\)}}} &
\textbf{\uline{0.6316 {\scriptsize\(\pm \ 0.0030\)}}} \\

\bottomrule

\multicolumn{11}{l}{\textsuperscript{1} We consider the early-stage analysis setting using the first 5 packets of each flow, which represents a constrained-setting comparison for hardware-offloadable models with longer observations.} \\

\end{tabular}%
}
\vspace{-12pt}
\end{table*}



\cg{We further evaluate \textit{Nepco} and baselines on three more network traffic datasets, i.e., CSTNET-20, CSTNET-120, and DoHBrw, which are adopted in recent network foundation model studies \cite{TrafficFormer-SP25,TrafficLLM-arXiv25}.
CSTNET-20 and CSTNET-120 are derived from the publicly available CSTNET-TLS1.3 \cite{ET-BERT-WWW22} dataset, which contains TLS 1.3-encrypted traffic from 120 mobile application classes.
Following the dataset settings of recent work, we use the complete dataset as CSTNET-120, and construct CSTNET-20 using the 20-class split released in the TrafficLLM repository \cite{TrafficLLM-arXiv25}.
DoHBrw \cite{DoHBrw-DASC20} contains four benign DNS-over-HTTPS (DoH) classes and one malicious DoH class.
Following the 5-class setting in TrafficLLM, we use it for the malicious DoH classification task.}

\cg{As shown in TABLE~\ref{tab:Additional Classification Performance}, \textit{Nepco} achieves competitive classification performance with existing network foundation models across the three network traffic datasets.
On CSTNET-20 and CSTNET-120, \textit{Nepco} achieves macro F1 scores of 0.8719 and 0.6457, improving upon the highest macro F1 scores achieved by existing network foundation models by 0.03\% and 4.30\%, respectively.
On DoHBrw, \textit{Nepco} achieves a macro F1 of 0.6316, which is 0.25\% lower than TrafficFormer’s 0.6332, the highest macro F1 among existing network foundation models.
Under the constrained early-stage analysis setting, \textit{Nepco} also consistently outperforms existing hardware-offloadable models across the three more datasets, improving macro F1 over Flowrest, Leo, Mousika, and BoS by 63.23\%, 695.72\%, 109.44\%, and 504.95\% on average, respectively.}


\subsection{\cg{Adversarial Robustness Evaluation}}

\label{Adversarial-Robustness}

\begin{figure}[t]
  \centering
  \includegraphics[width=1\linewidth]{Fig/Robustness/V2.pdf}
  \caption{\cg{Adversarial robustness evaluation of \textit{Nepco} and three Transformer-based network foundation models.}}
  \vspace{-8pt}
  \label{fig:Robustness}
\end{figure}


\cg{We conduct the adversarial robustness evaluation experiment on the CIC-EVSE dataset and compare \textit{Nepco} with three Transformer-based network foundation models, i.e., ET-BERT, TraGe, and TrafficFormer. For each model, we first train a model using the unperturbed training set. Based on the trained model, we apply gradient-based attribution \cite{gradient-arXiv17} to each sample in the training and test sets and rank its input bytes according to their attribution scores. We then construct two byte-level perturbation strategies. Random-X\% perturbation randomly selects X\% of the input bytes, while Top-X\% perturbation selects the top X\% most important bytes according to the byte importance ranking. Under both strategies, the selected bytes are replaced with random byte values. Based on the perturbed training and test sets, we consider four evaluation settings:}

\begin{itemize}[leftmargin=*]
\item \cg{\textbf{Raw-Random}: The model is trained on the unperturbed raw training set and evaluated on the Random-X\% test set.}
\item \cg{\textbf{Raw-Top}: The model is trained on the unperturbed raw training set and evaluated on the Top-X\% test set.}
\item \cg{\textbf{Random-Random}: The model is trained on the Random-X\% training set and evaluated on the Random-X\% test set.}
\item \cg{\textbf{Top-Top}: The model is trained on the Top-X\% training set and evaluated on the Top-X\% test set.}
\end{itemize}

\cg{The dashed lines in Fig. \ref{fig:Robustness} show the macro F1 of different models when the test samples are perturbed by Random-X\% and Top-X\% perturbations, corresponding to the Raw-Random and Raw-Top settings, respectively, while the gray lines show the macro F1 when the test samples are not perturbed.
Under Random-X\% perturbation, the macro F1 degradation is limited. Over the perturbation range from 0\% to 5\%, each 1-percentage-point increase in X corresponds to average macro F1 reductions of 0.0098, 0.0143, 0.0096, and 0.0037 for \textit{Nepco}, TrafficFormer, TraGe, and ET-BERT, respectively.
Under Top-X\% perturbation, the macro F1 decreases substantially as X increases, with corresponding average reductions of 0.0878, 0.0951, 0.0951, and 0.0953.
These results show that the four models are sensitive to perturbations of high-importance bytes, while \textit{Nepco} does not exhibit greater sensitivity than the three Transformer-based models.}

\cg{The solid lines in Fig. \ref{fig:Robustness} show the macro F1 of different models when both the training and test samples are perturbed by Random-X\% and Top-X\% perturbations, corresponding to the Random-Random and Top-Top settings, respectively.
Under both strategies, introducing the corresponding perturbations during training substantially mitigates the performance degradation caused by test-time perturbations, with the four models maintaining macro F1 above 0.84 across the evaluated perturbation ratios.
Specifically, under Top-5\% perturbation, the macro F1 of \textit{Nepco}, TrafficFormer, TraGe, and ET-BERT are 0.8447, 0.9082, 0.8987, and 0.8918, respectively.}
